# Supplementary material for: Auto-FP: An Experimental Study of Automated Feature Preprocessing for Tabular Data
Source: arXiv:2310.02540 source file (2026-04-15)
Supplement: Supplementary file 1 [file appendix.tex]

\begin{appendix}

\section{1}
\begin{figure*}[htbp]
\centering
\subfigure[Austrilian, LR]{
\label{Fig.sub.1}
\includegraphics[width=0.18\textwidth]{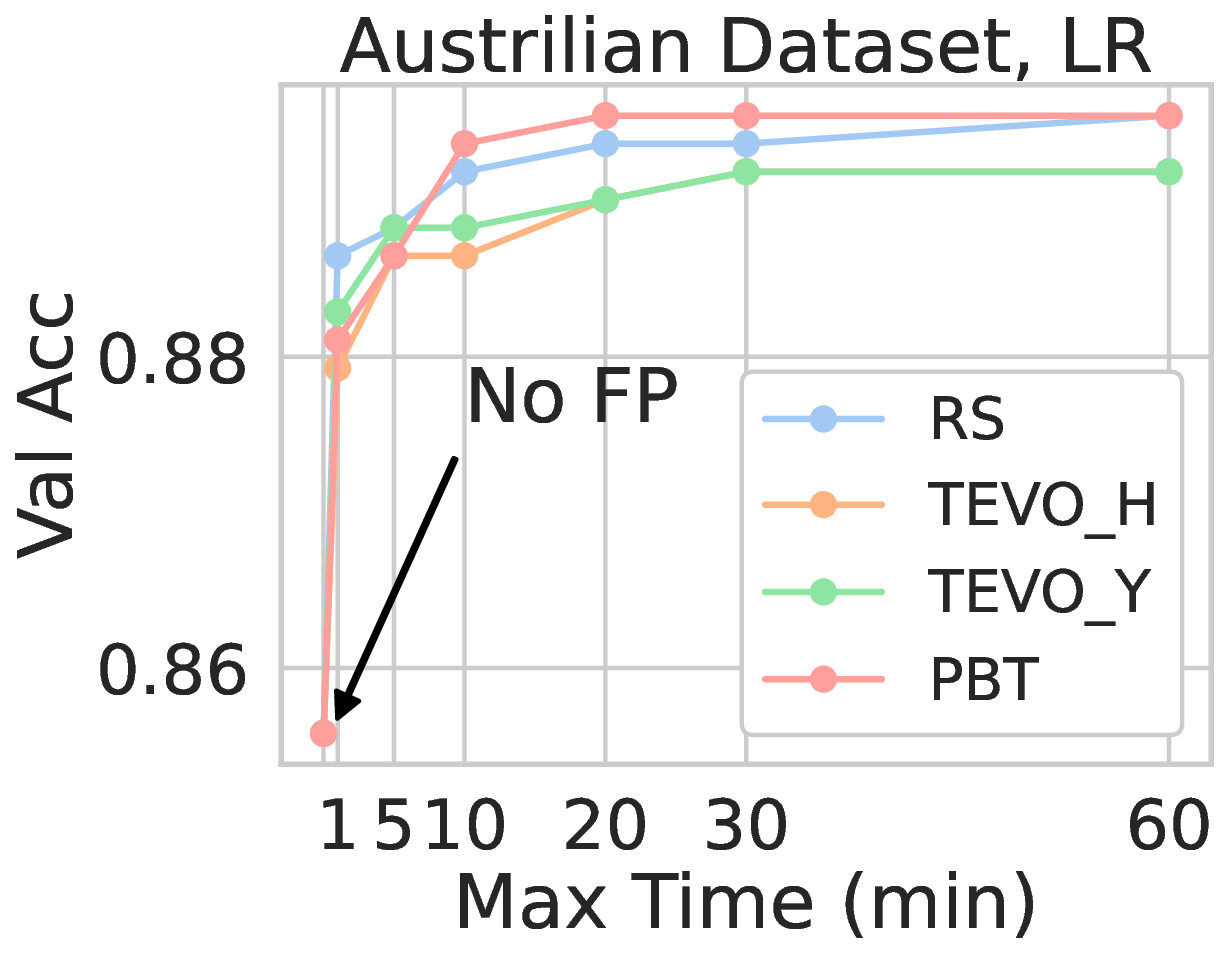}}
\subfigure[Blood, LR]{
\label{Fig.sub.2}
\includegraphics[width=0.18\textwidth]{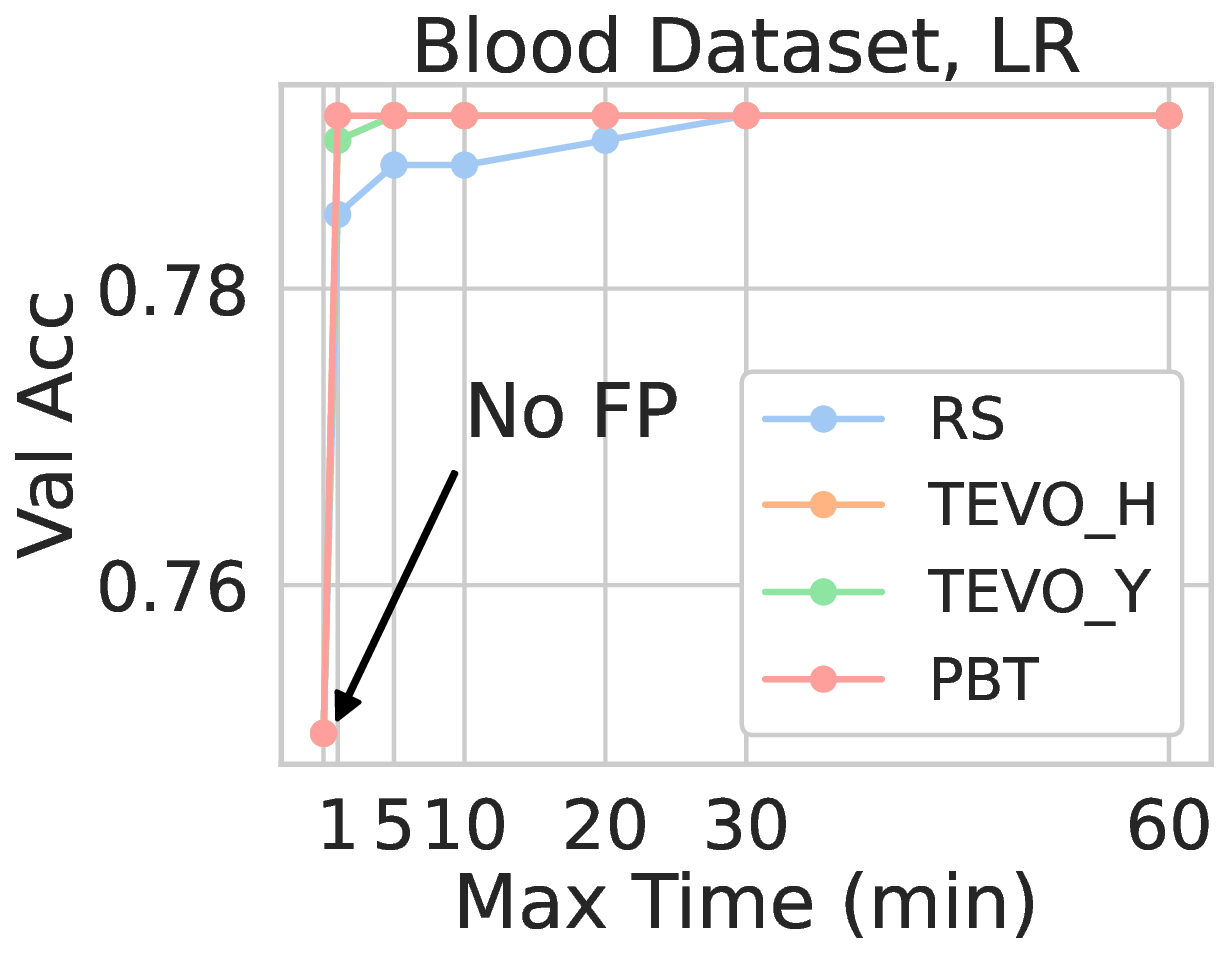}}
\subfigure[Emotion, LR]{
\label{Fig.sub.3}
\includegraphics[width=0.18\textwidth]{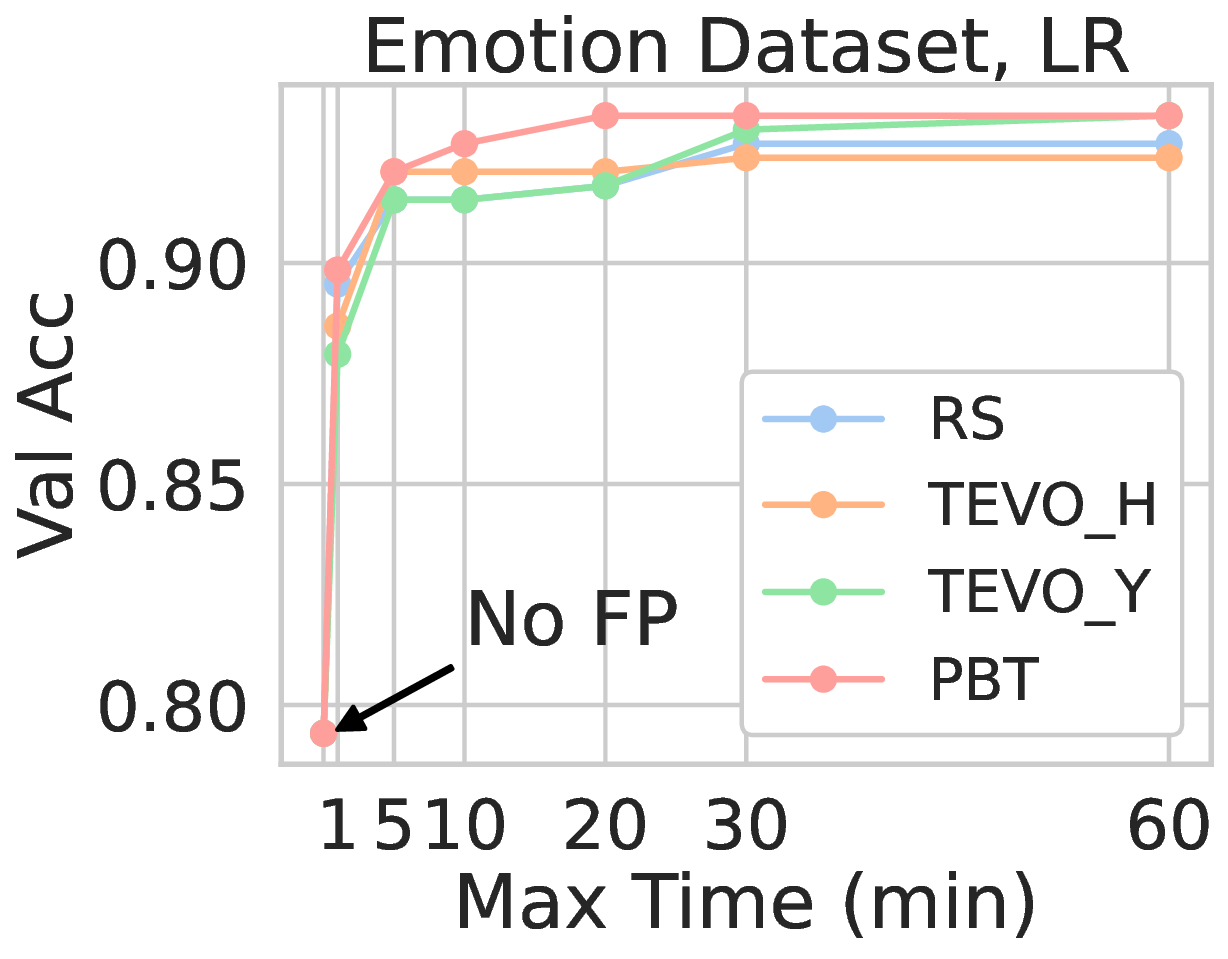}}
\subfigure[Heart, LR]{
\label{Fig.sub.4}
\includegraphics[width=0.18\textwidth]{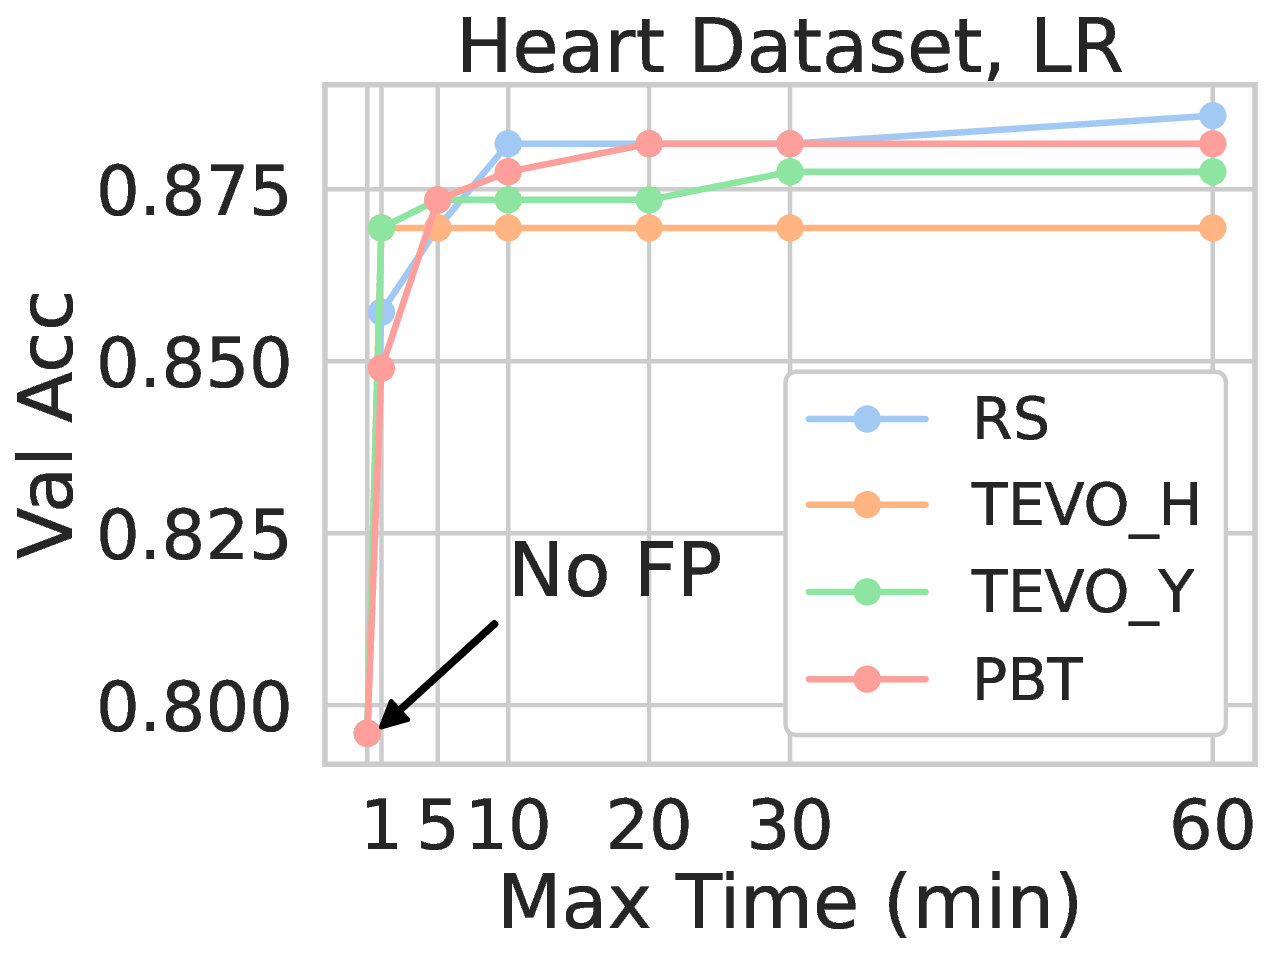}}
\subfigure[Forex, LR]{
\label{Fig.sub.5}
\includegraphics[width=0.18\textwidth]{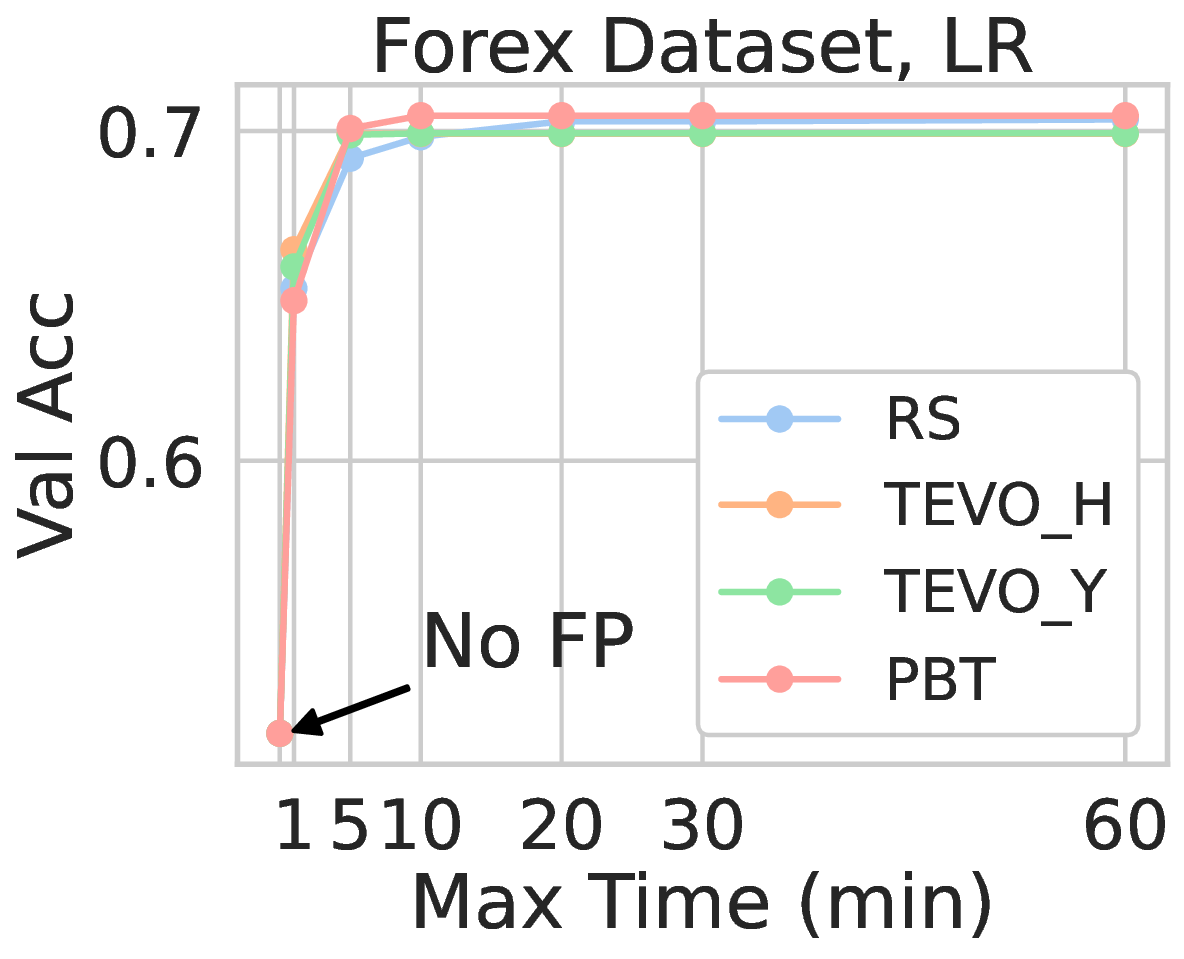}}

\subfigure[Austrilian, XGB]{
\label{Fig.sub.1}
\includegraphics[width=0.18\textwidth]{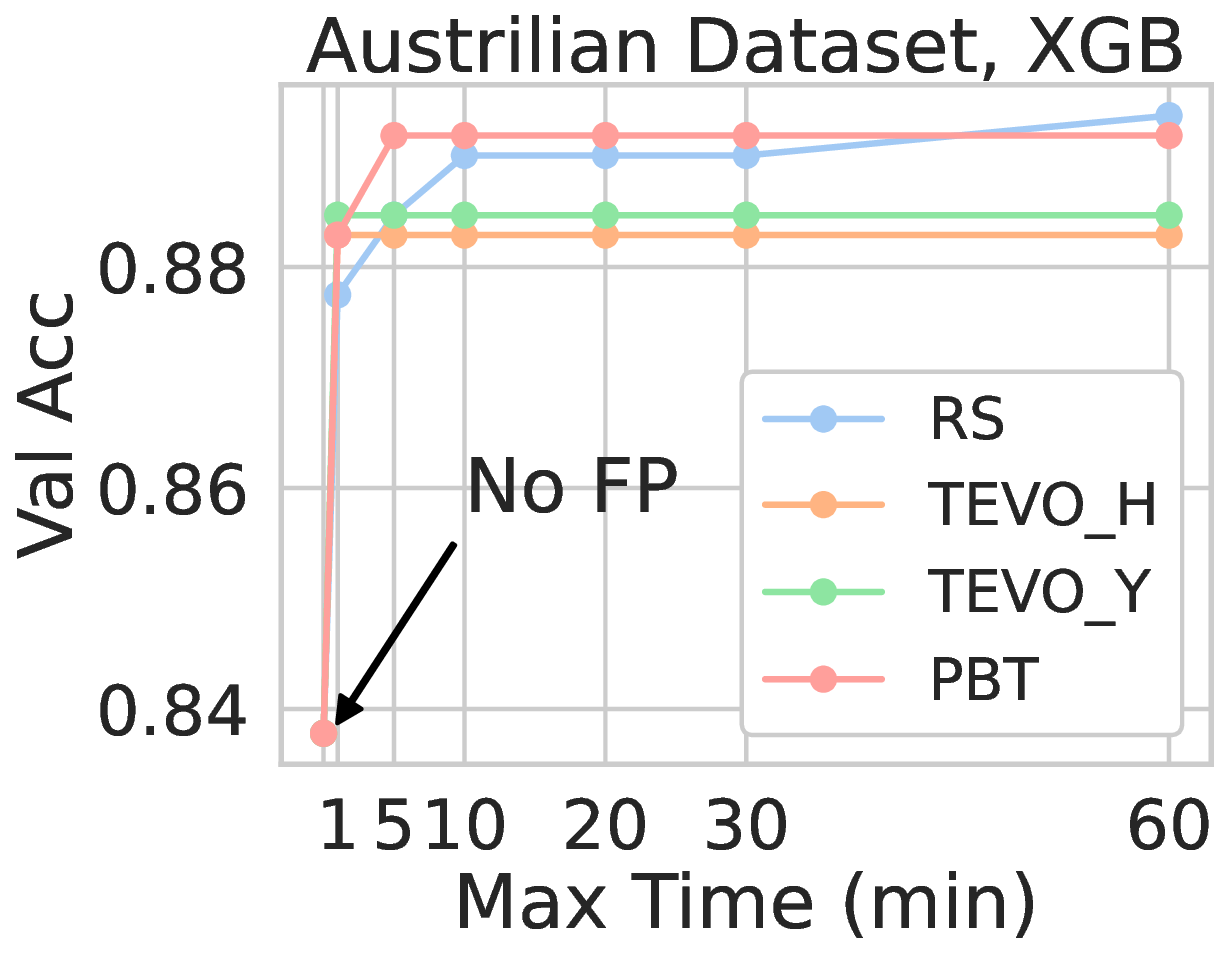}}
\subfigure[Blood, XGB]{
\label{Fig.sub.2}
\includegraphics[width=0.18\textwidth]{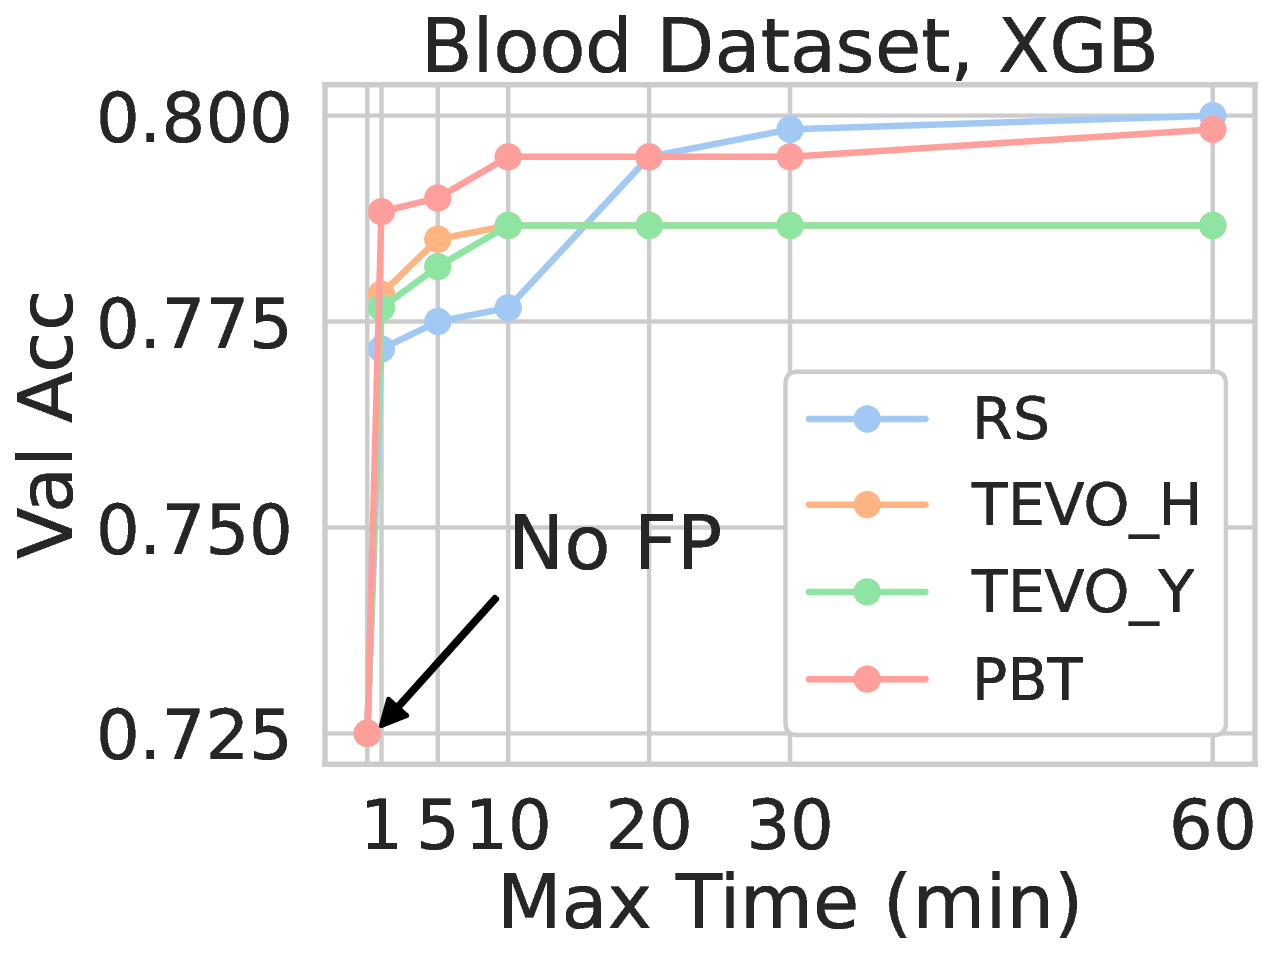}}
\subfigure[Emotion, XGB]{
\label{Fig.sub.3}
\includegraphics[width=0.18\textwidth]{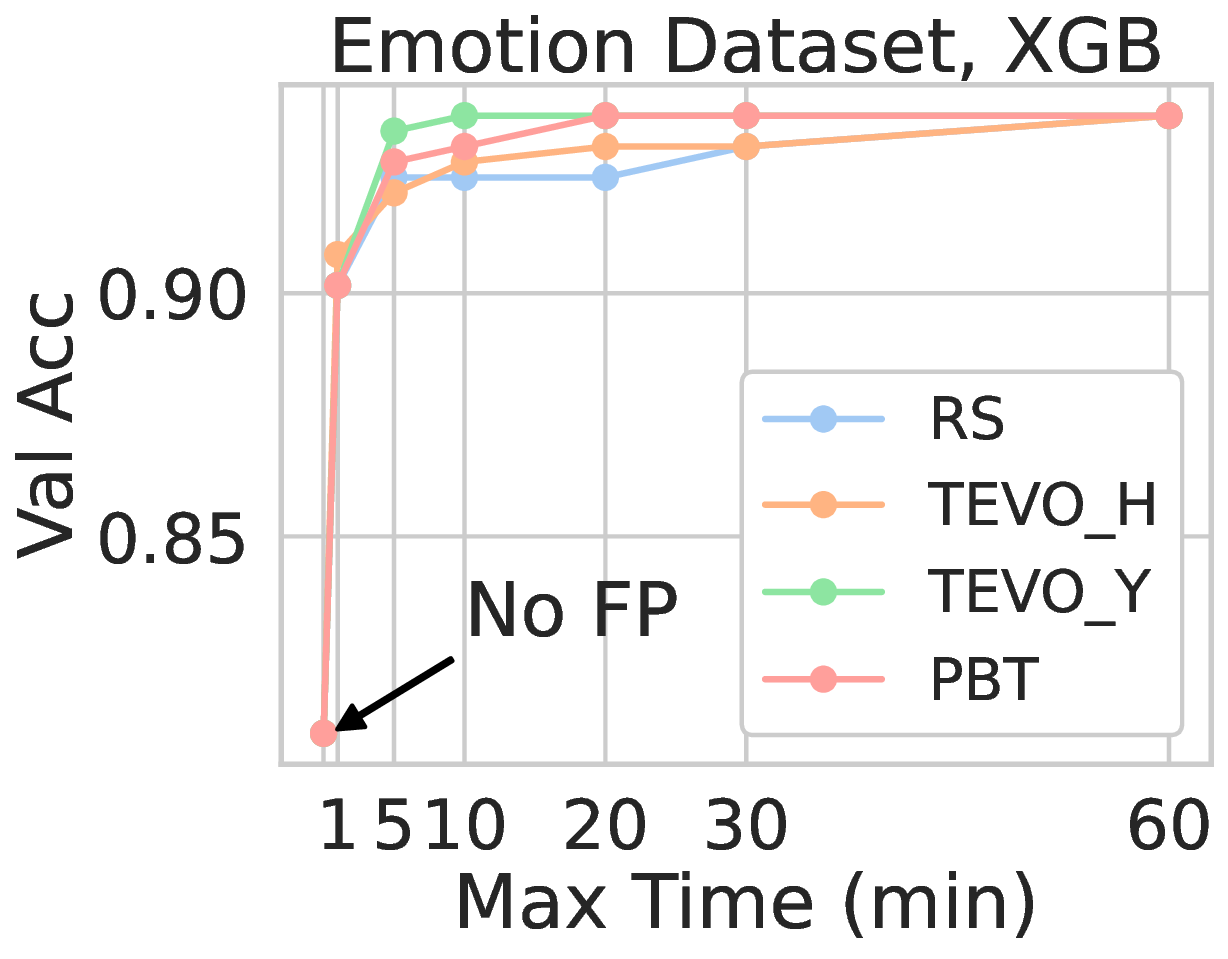}}
\subfigure[Heart, XGB]{
\label{Fig.sub.4}
\includegraphics[width=0.18\textwidth]{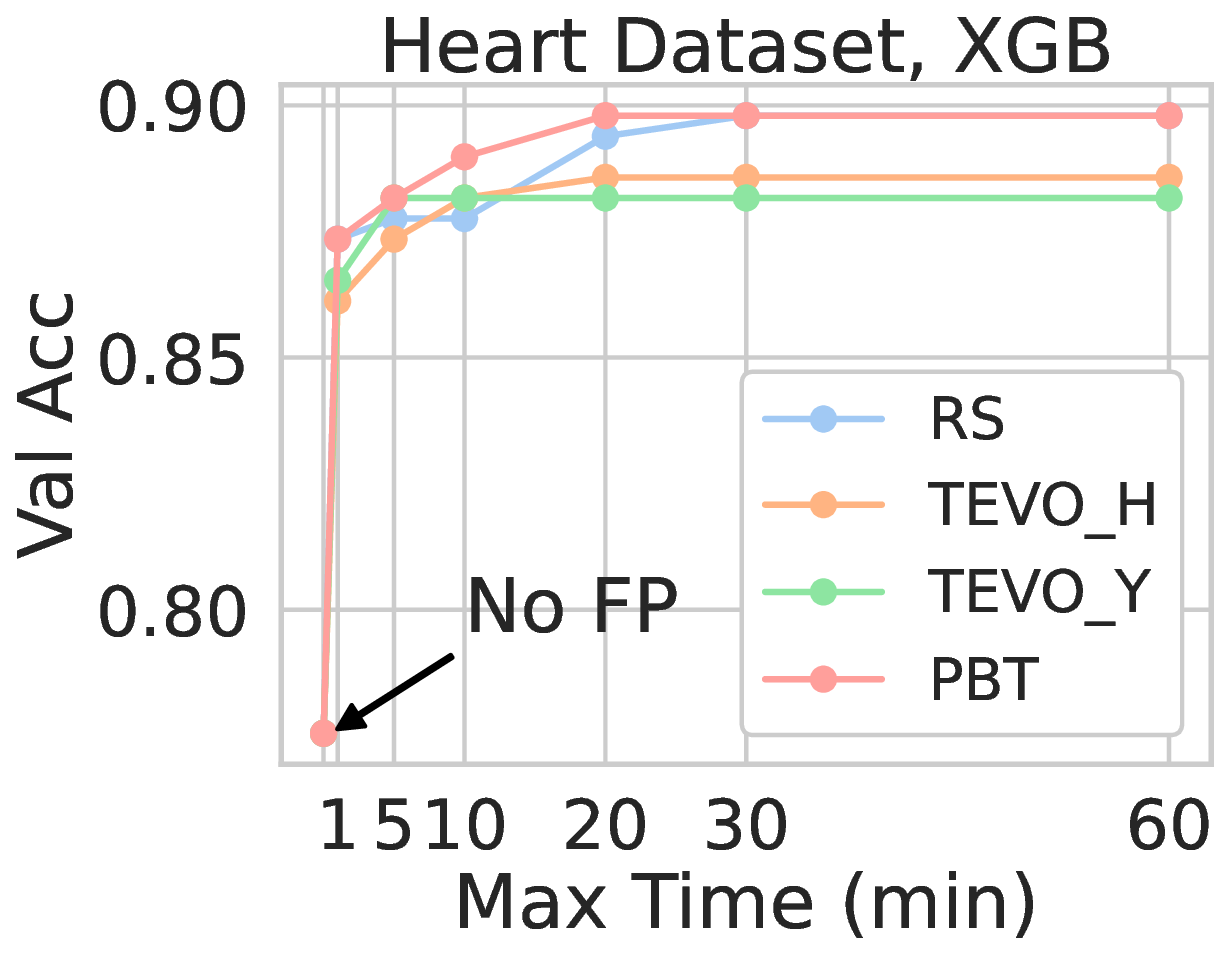}}
\subfigure[Forex, XGB]{
\label{Fig.sub.5}
\includegraphics[width=0.18\textwidth]{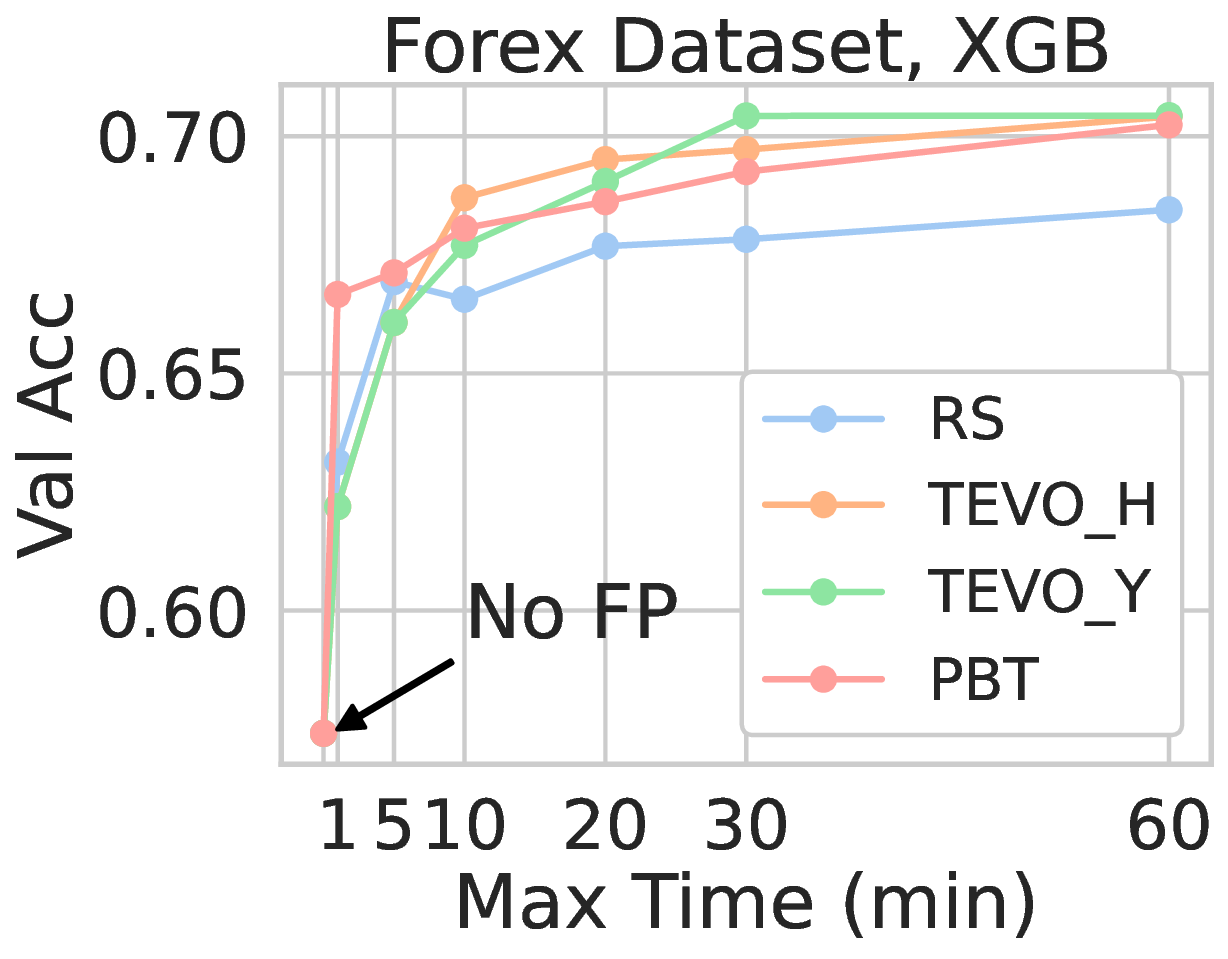}}

\subfigure[Austrilian, MLP]{
\label{Fig.sub.1}
\includegraphics[width=0.18\textwidth]{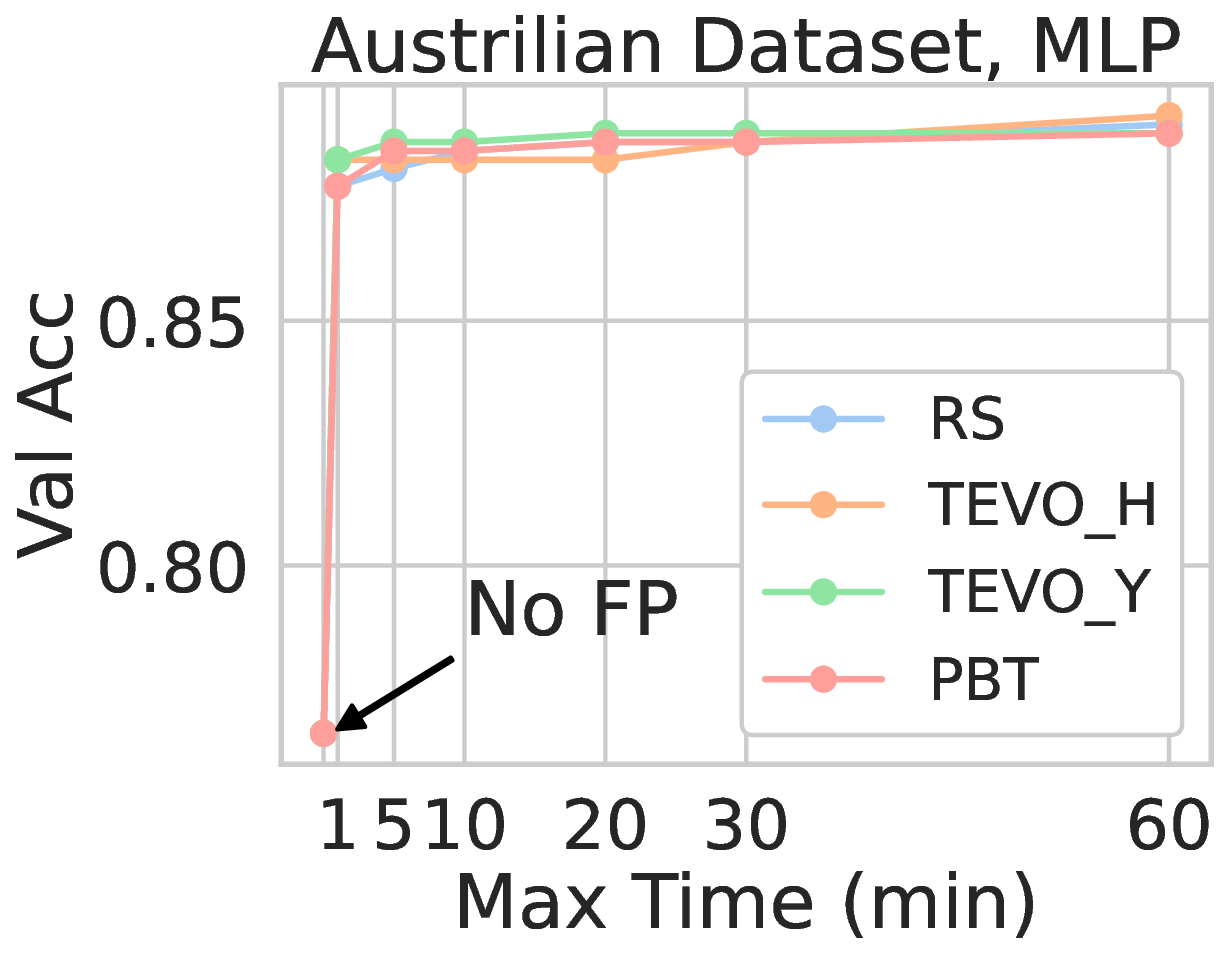}}
\subfigure[Blood, MLP]{
\label{Fig.sub.2}
\includegraphics[width=0.18\textwidth]{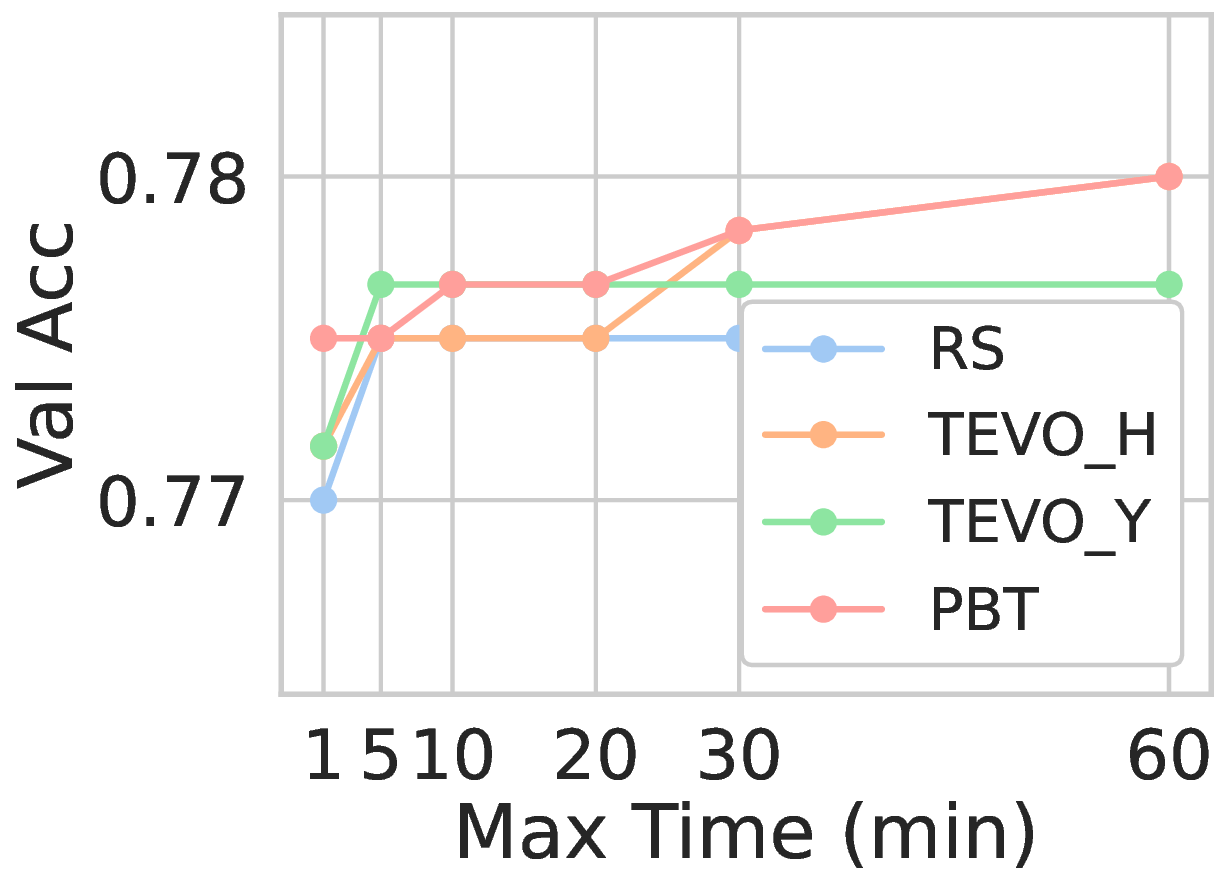}}
\subfigure[Emotion, MLP]{
\label{Fig.sub.3}
\includegraphics[width=0.18\textwidth]{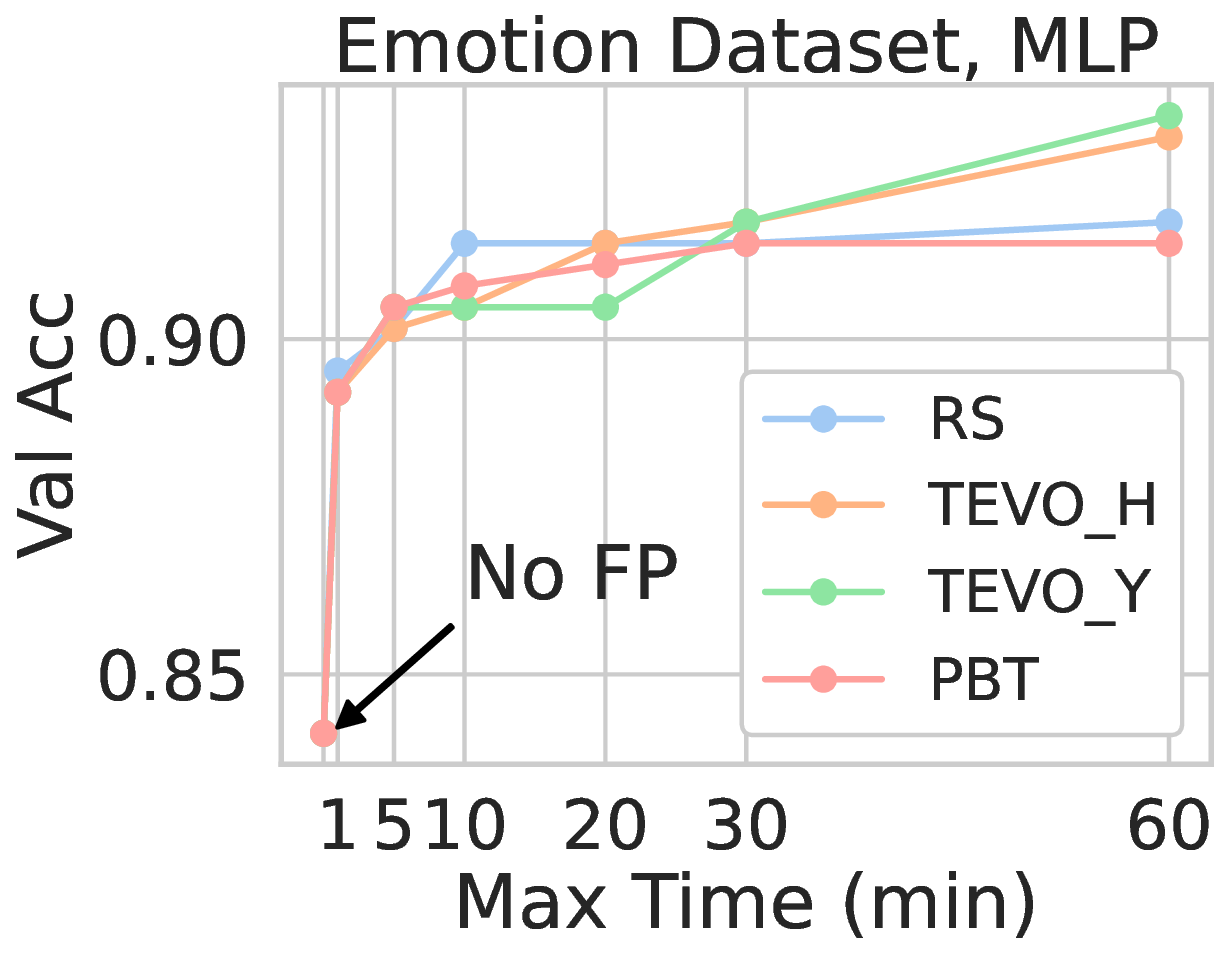}}
\subfigure[Heart, MLP]{
\label{Fig.sub.4}
\includegraphics[width=0.18\textwidth]{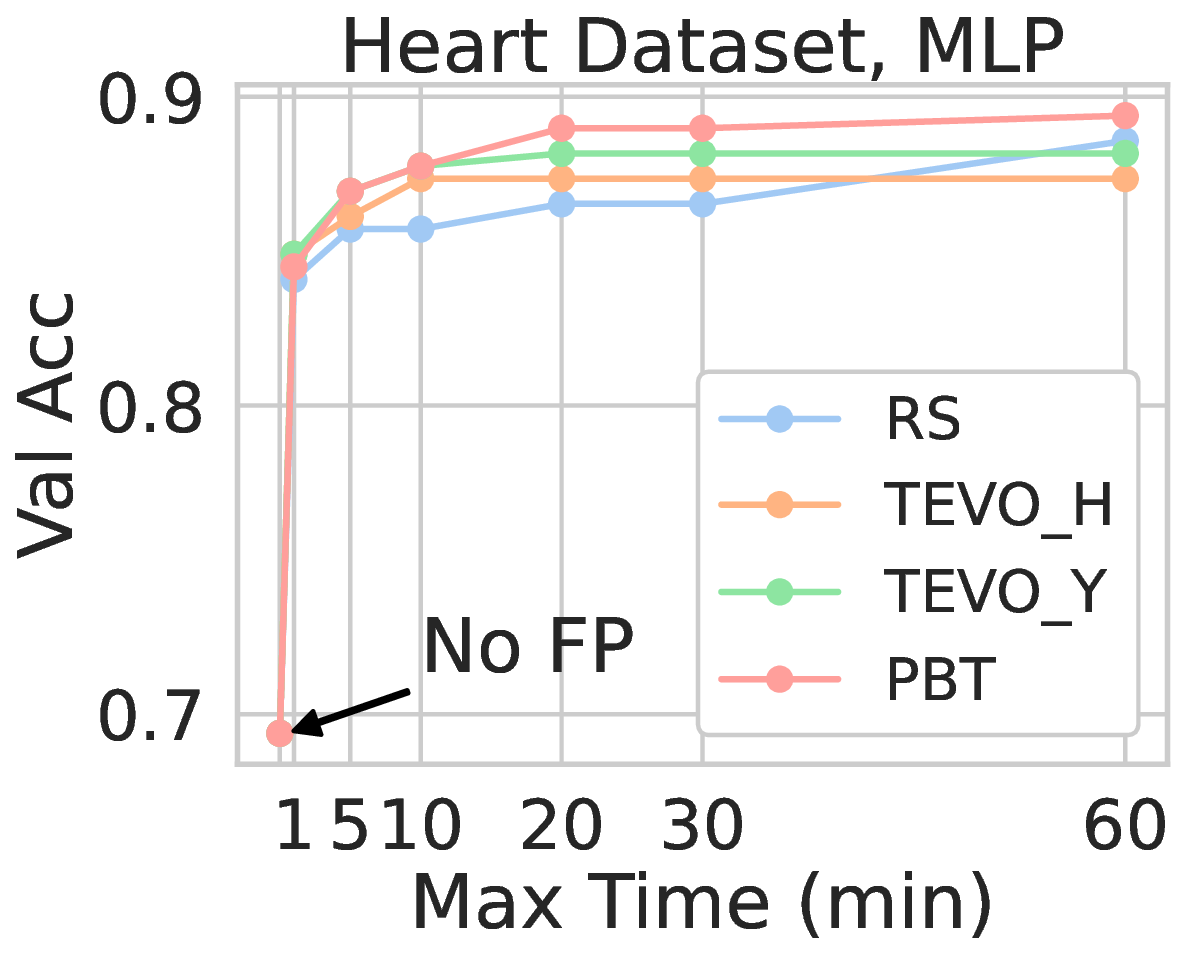}}
\subfigure[Forex, MLP]{
\label{Fig.sub.5}
\includegraphics[width=0.18\textwidth]{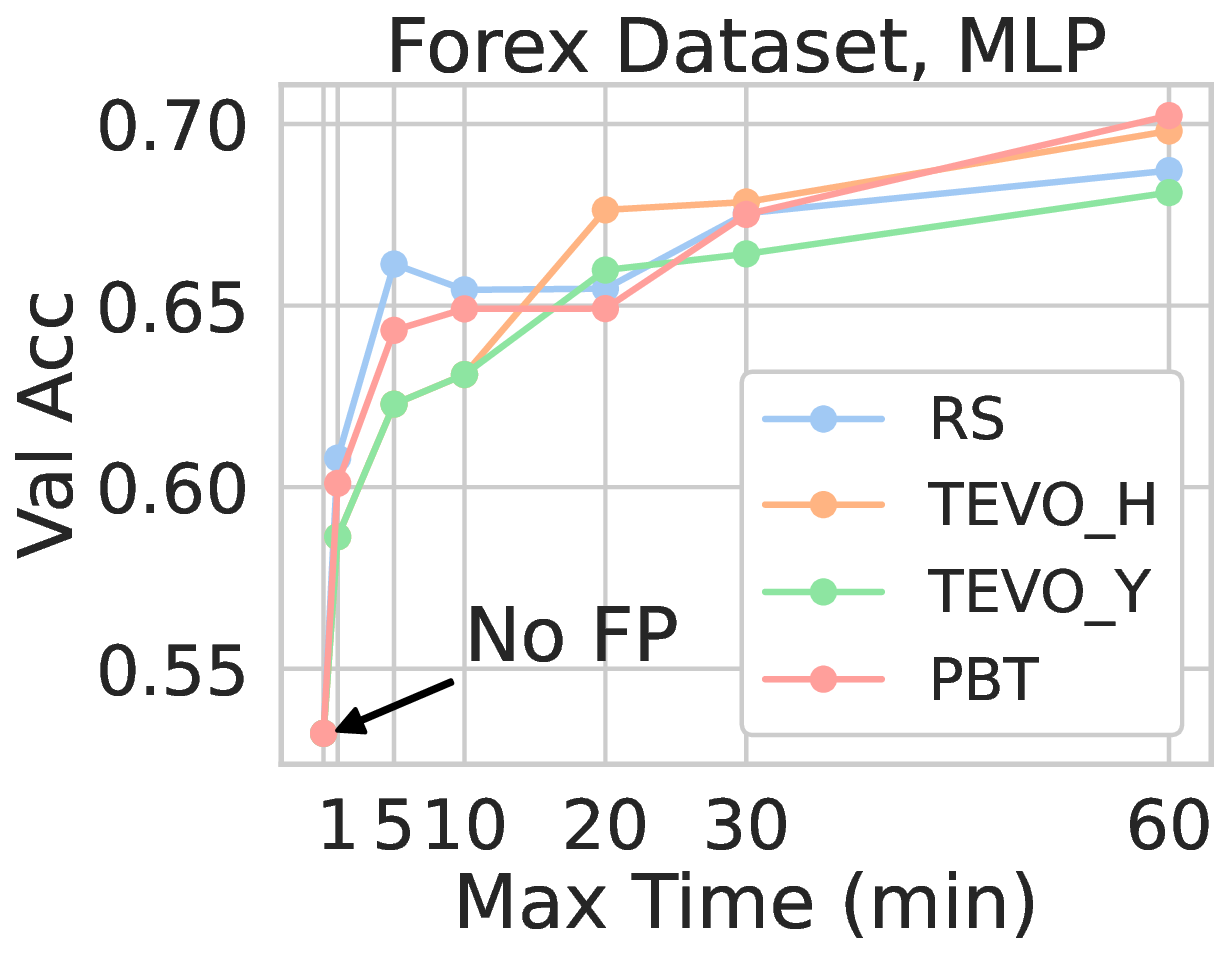}}

\subfigure[Jasmine, LR]{
\label{Fig.sub.1}
\includegraphics[width=0.18\textwidth]{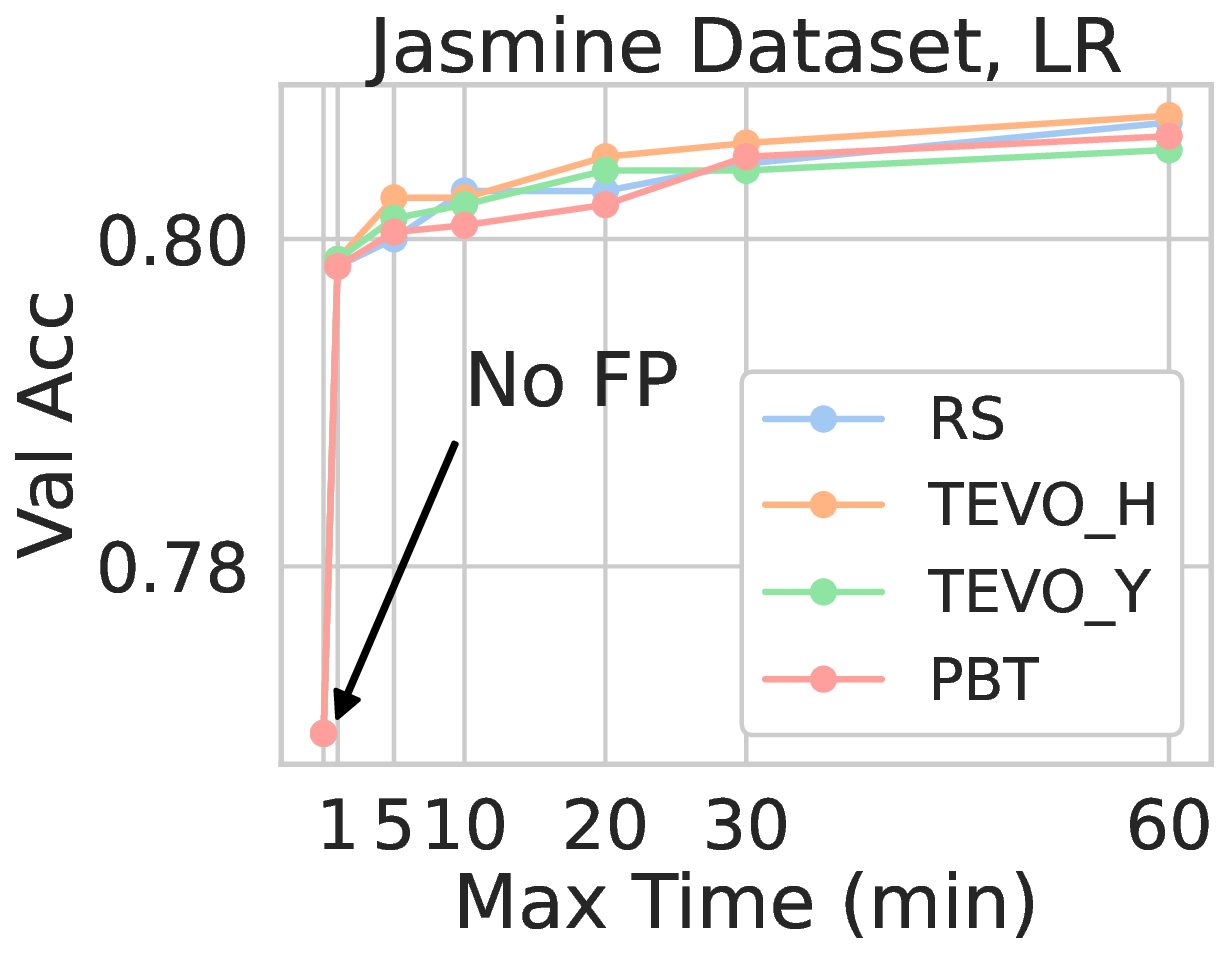}}
\subfigure[Madeline, LR]{
\label{Fig.sub.2}
\includegraphics[width=0.18\textwidth]{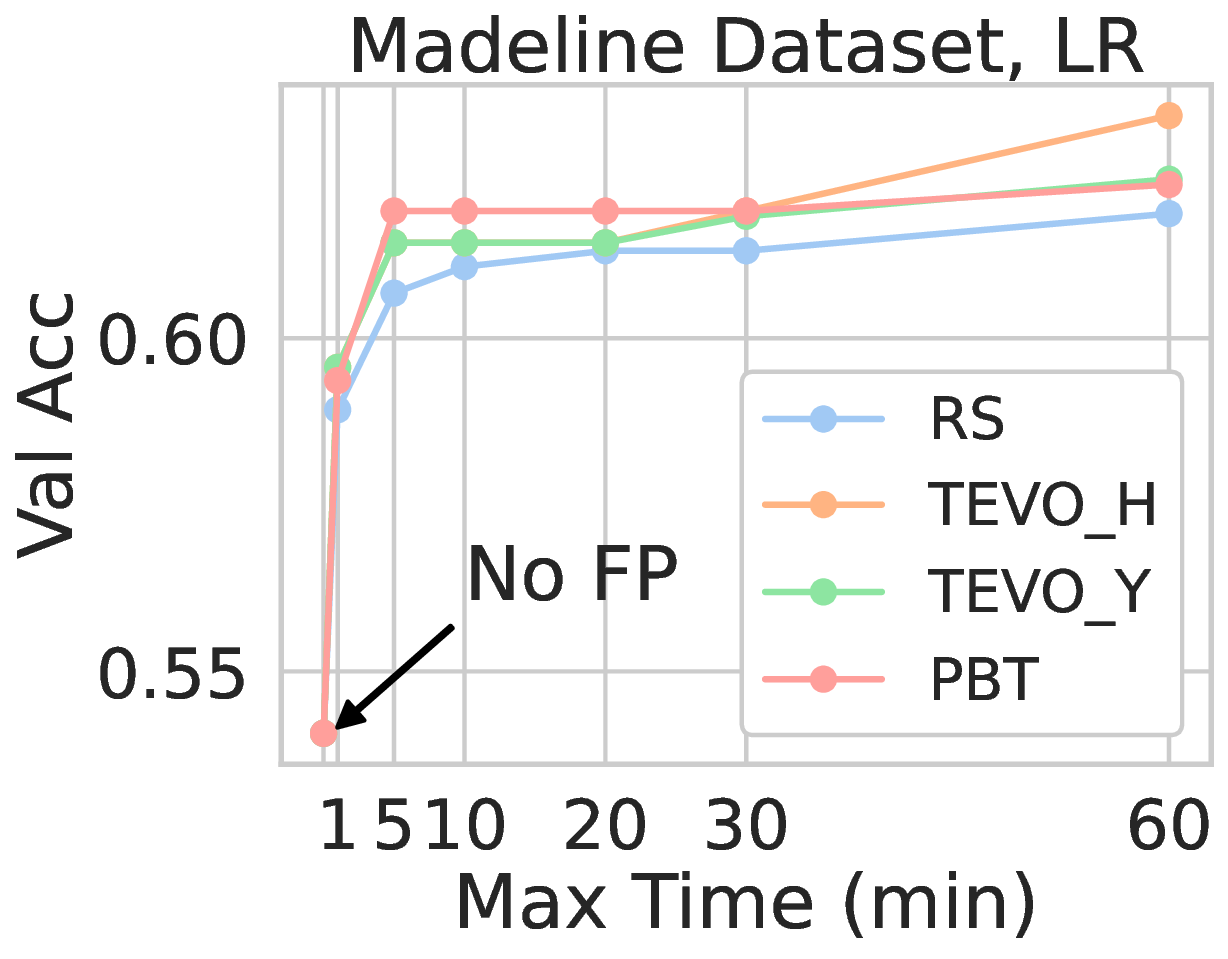}}
\subfigure[Pd\_speech\_features, LR]{
\label{Fig.sub.3}
\includegraphics[width=0.18\textwidth]{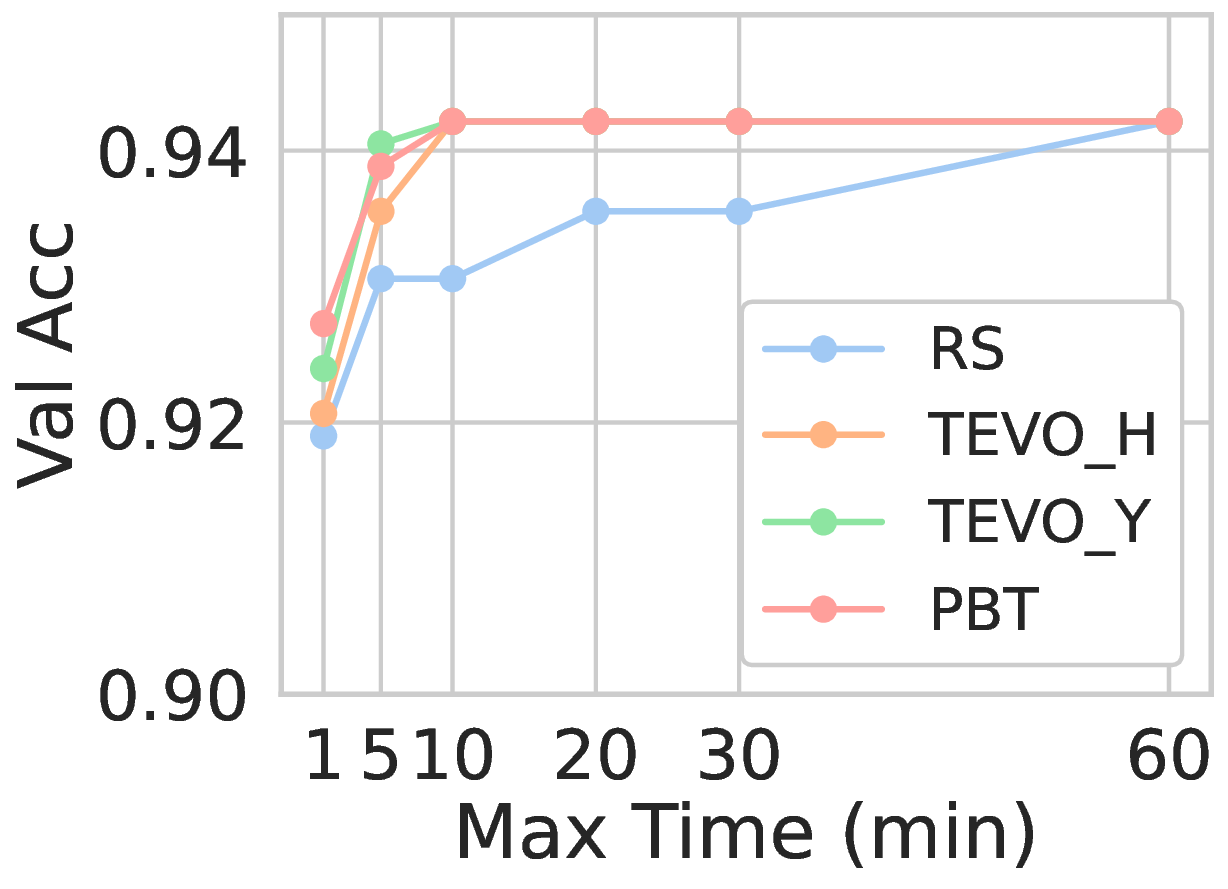}}
\subfigure[Wine\_quality, LR]{
\label{Fig.sub.4}
\includegraphics[width=0.18\textwidth]{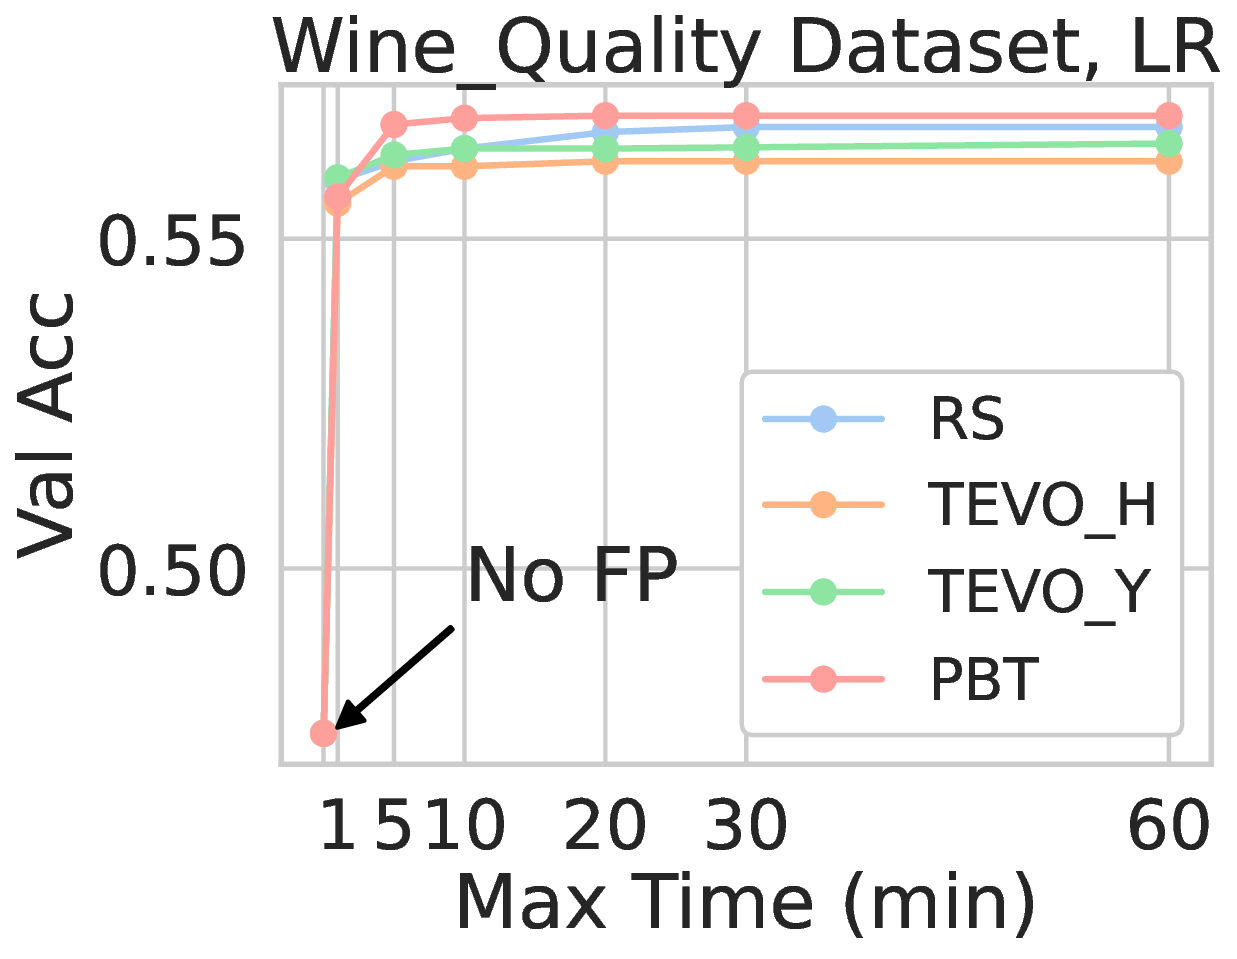}}
\subfigure[Thyroid\_allhyper, LR]{
\label{Fig.sub.5}
\includegraphics[width=0.18\textwidth]{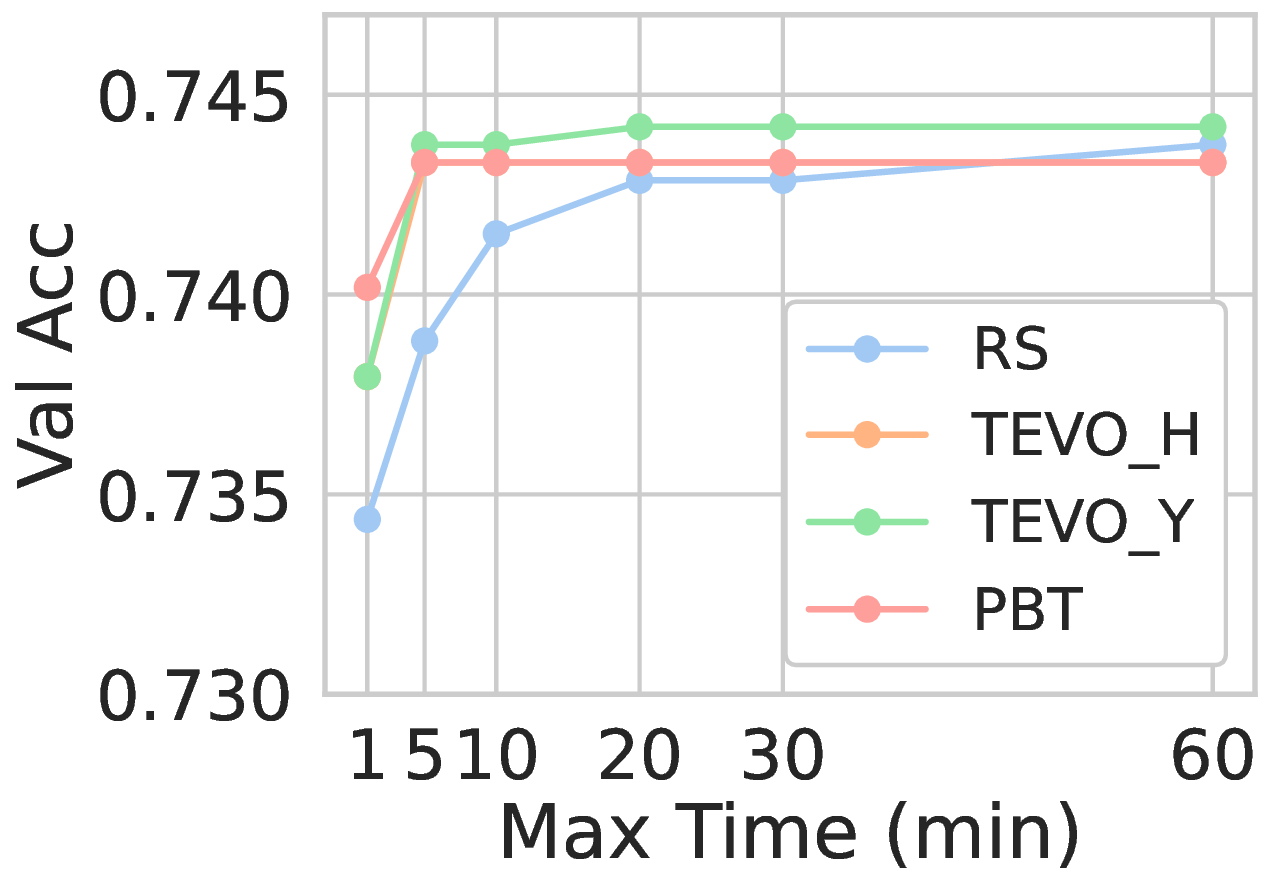}}

\subfigure[Jasmine, XGB]{
\label{Fig.sub.1}
\includegraphics[width=0.18\textwidth]{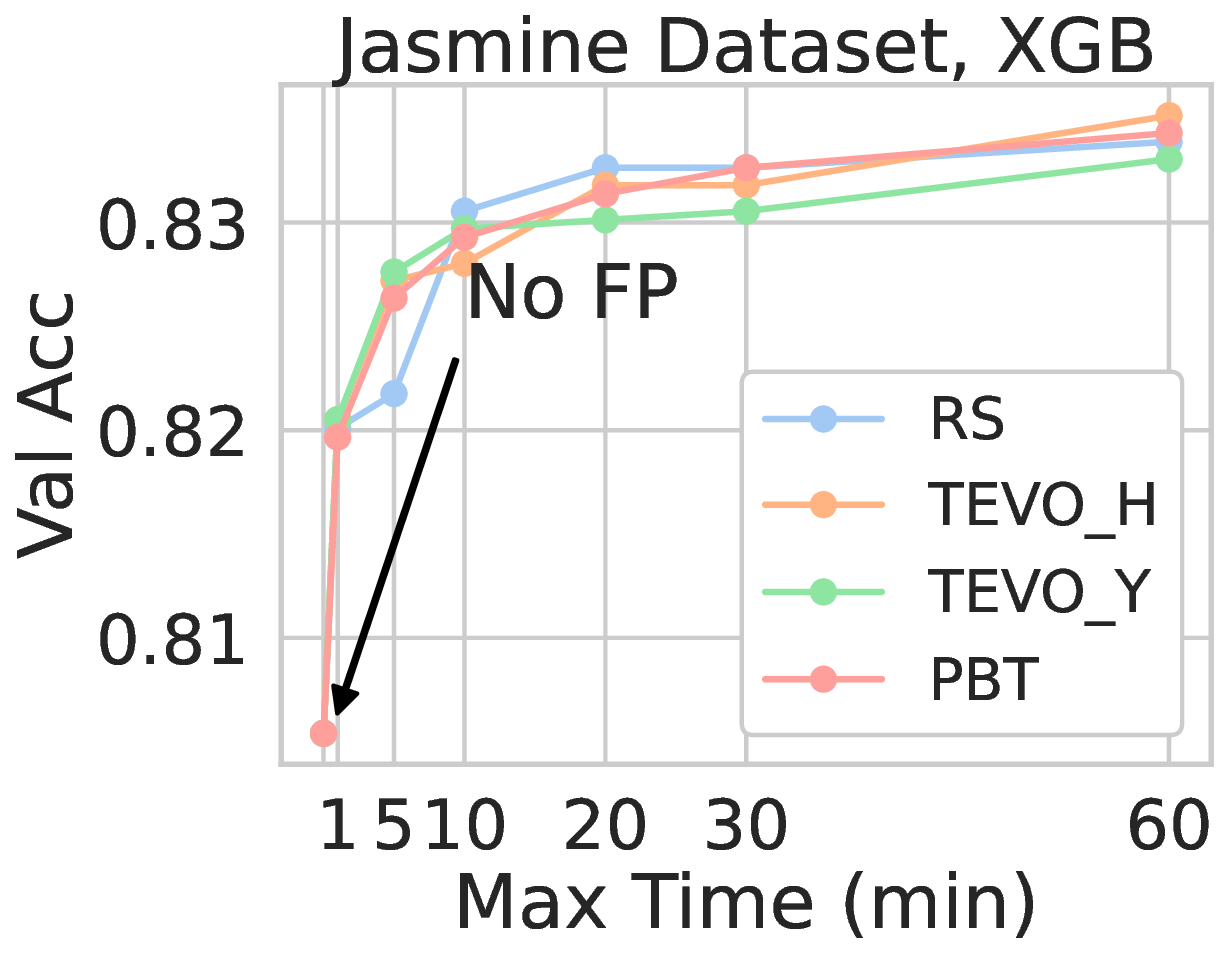}}
\subfigure[Madeline, XGB]{
\label{Fig.sub.2}
\includegraphics[width=0.18\textwidth]{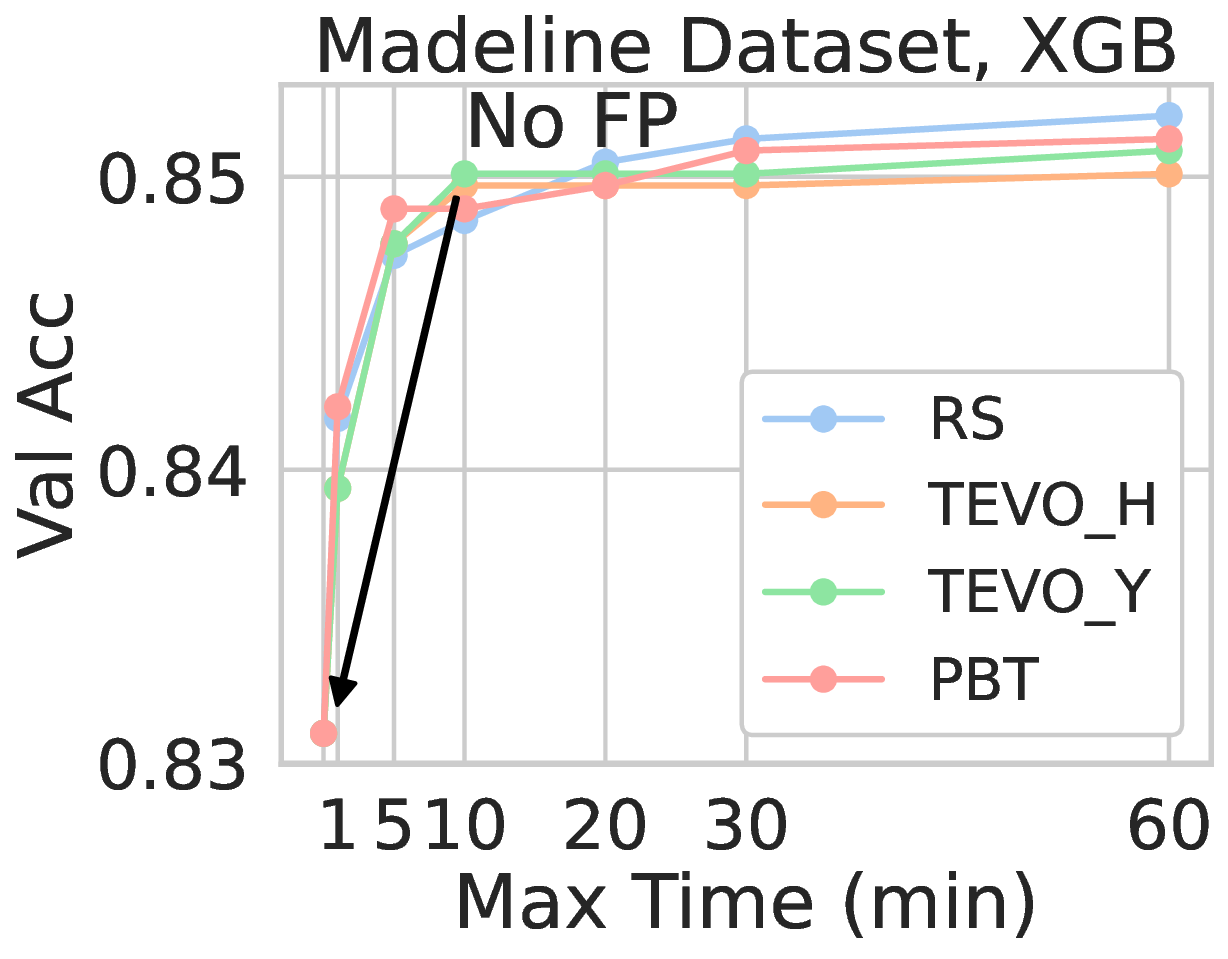}}
\subfigure[Pd\_speech\_features, XGB]{
\label{Fig.sub.3}
\includegraphics[width=0.18\textwidth]{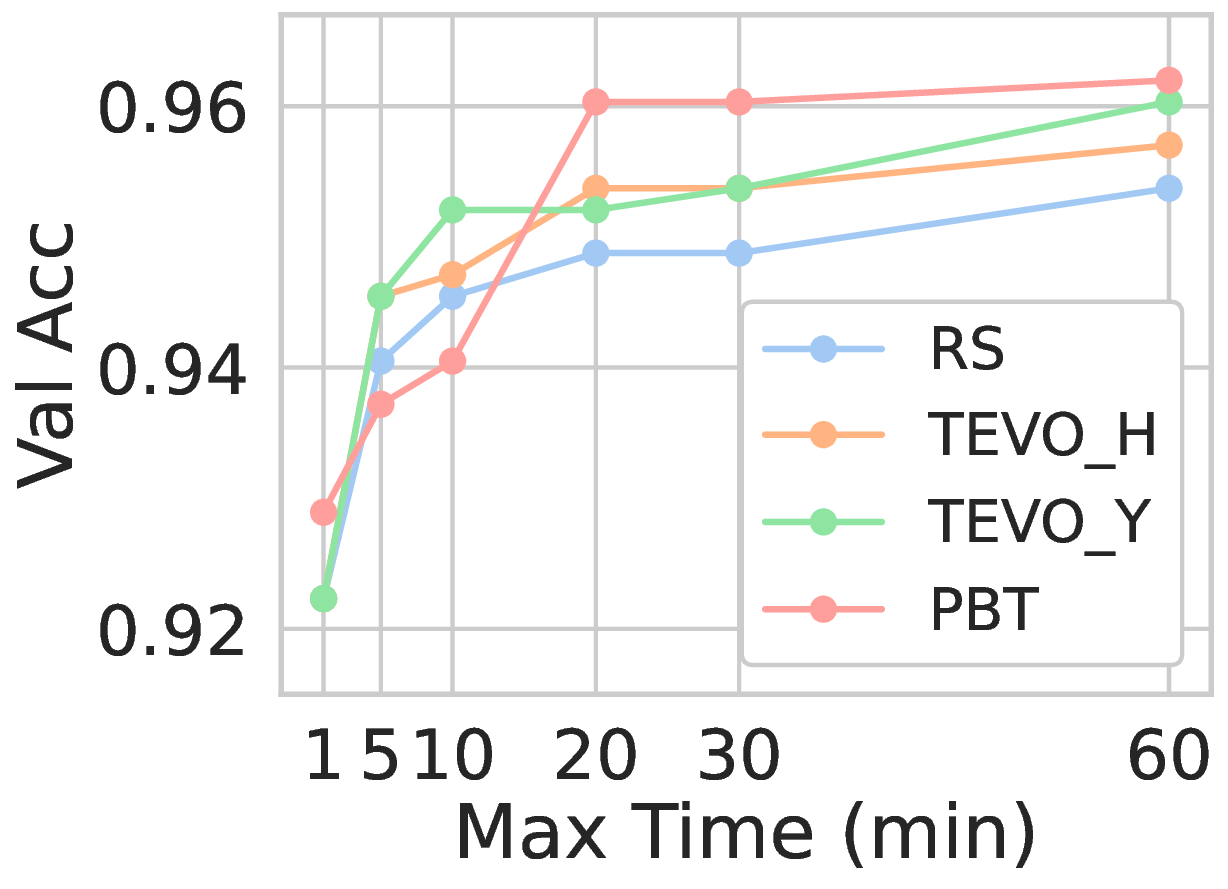}}
\subfigure[Wine\_quality, XGB]{
\label{Fig.sub.4}
\includegraphics[width=0.18\textwidth]{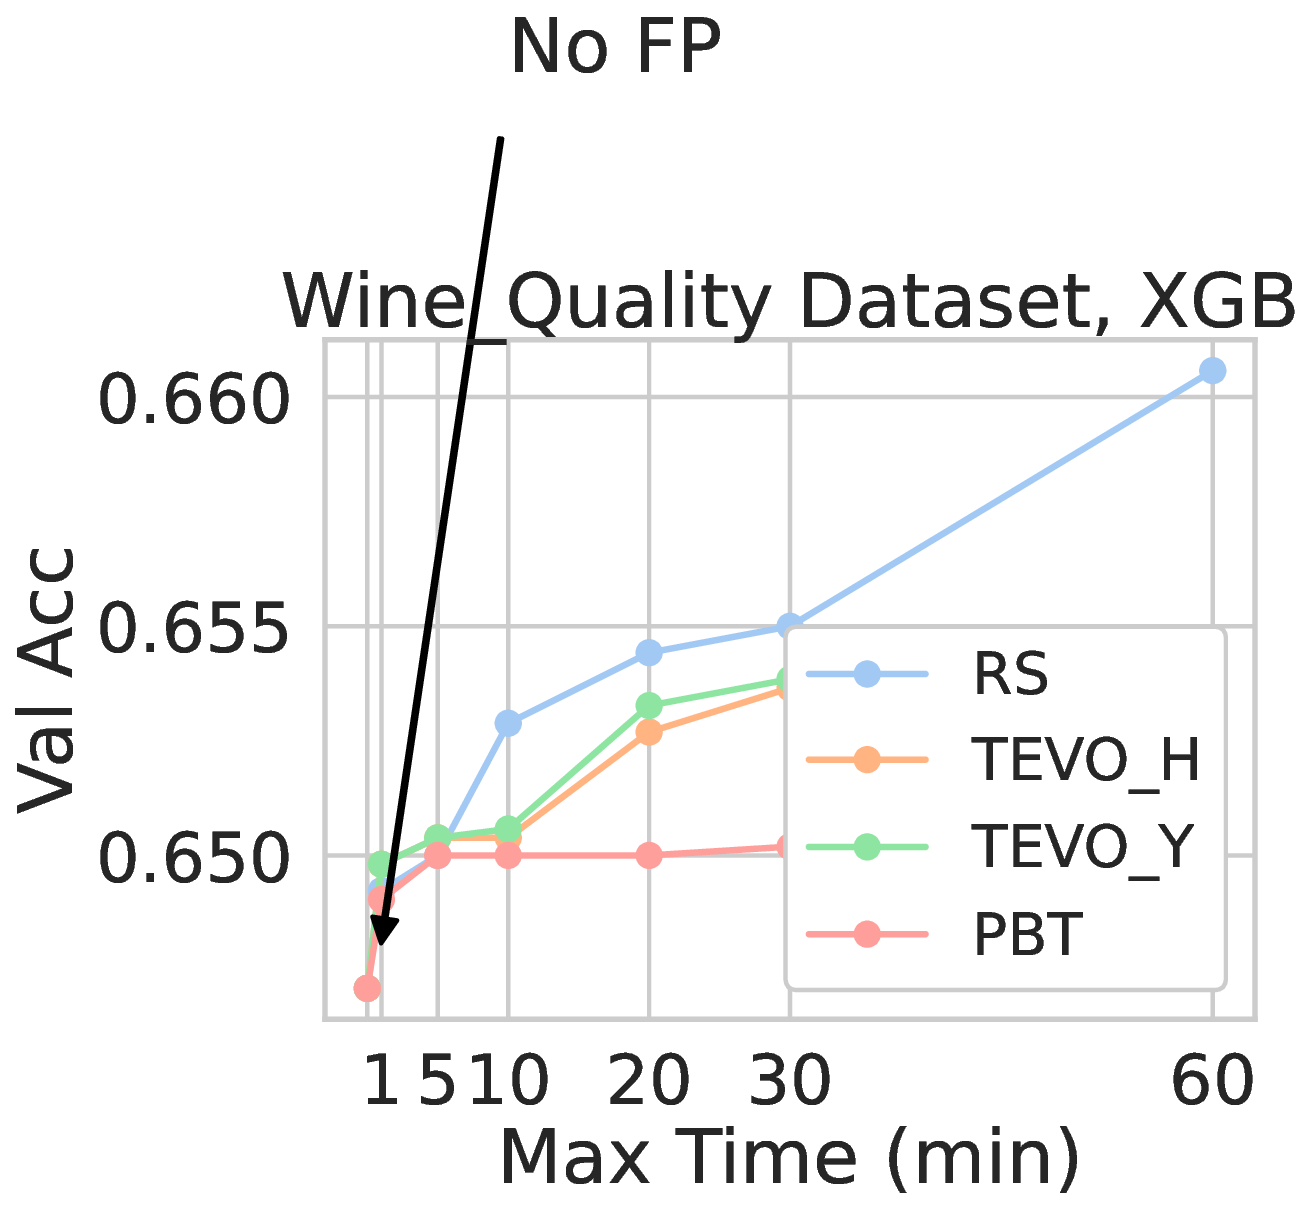}}
\subfigure[Thyroid\_allhyper, XGB]{
\label{Fig.sub.5}
\includegraphics[width=0.18\textwidth]{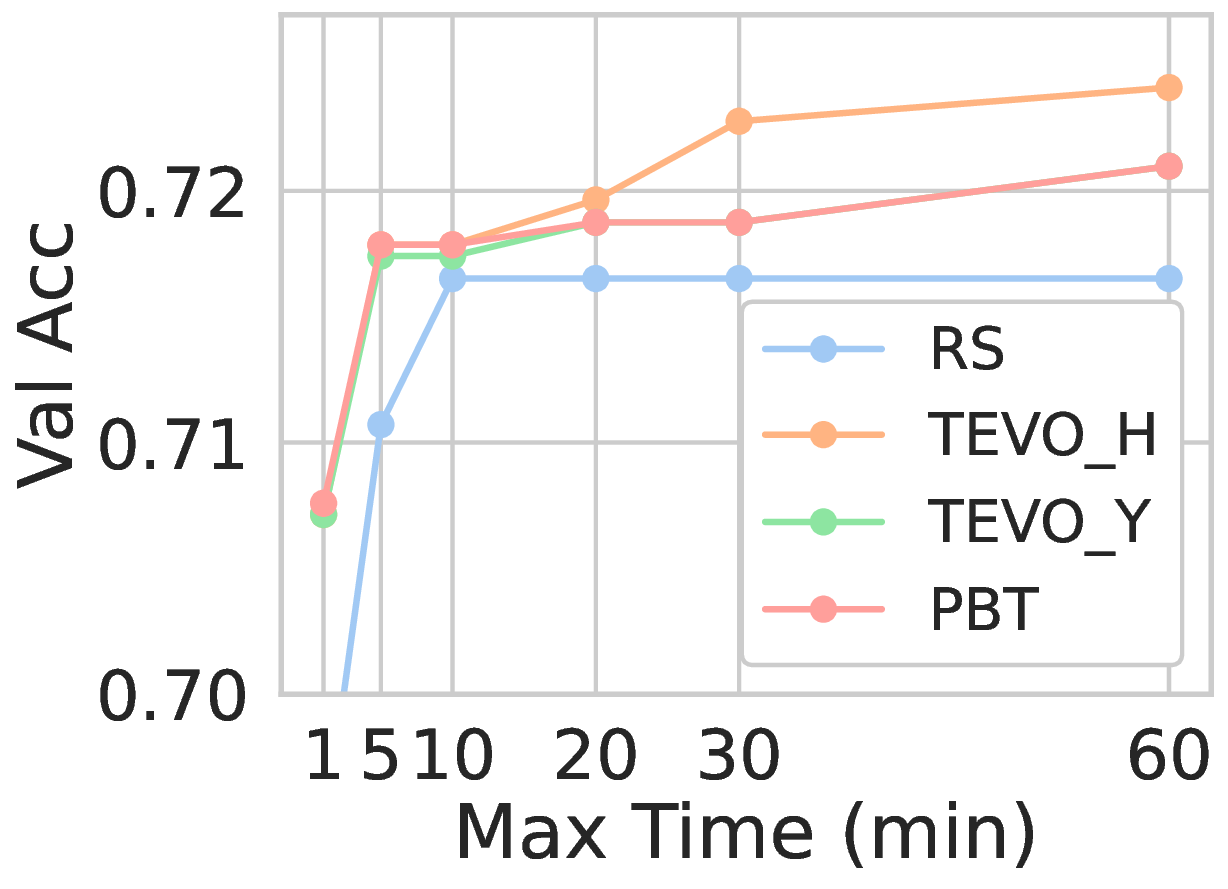}}

\subfigure[Jasmine, MLP]{
\label{Fig.sub.1}
\includegraphics[width=0.18\textwidth]{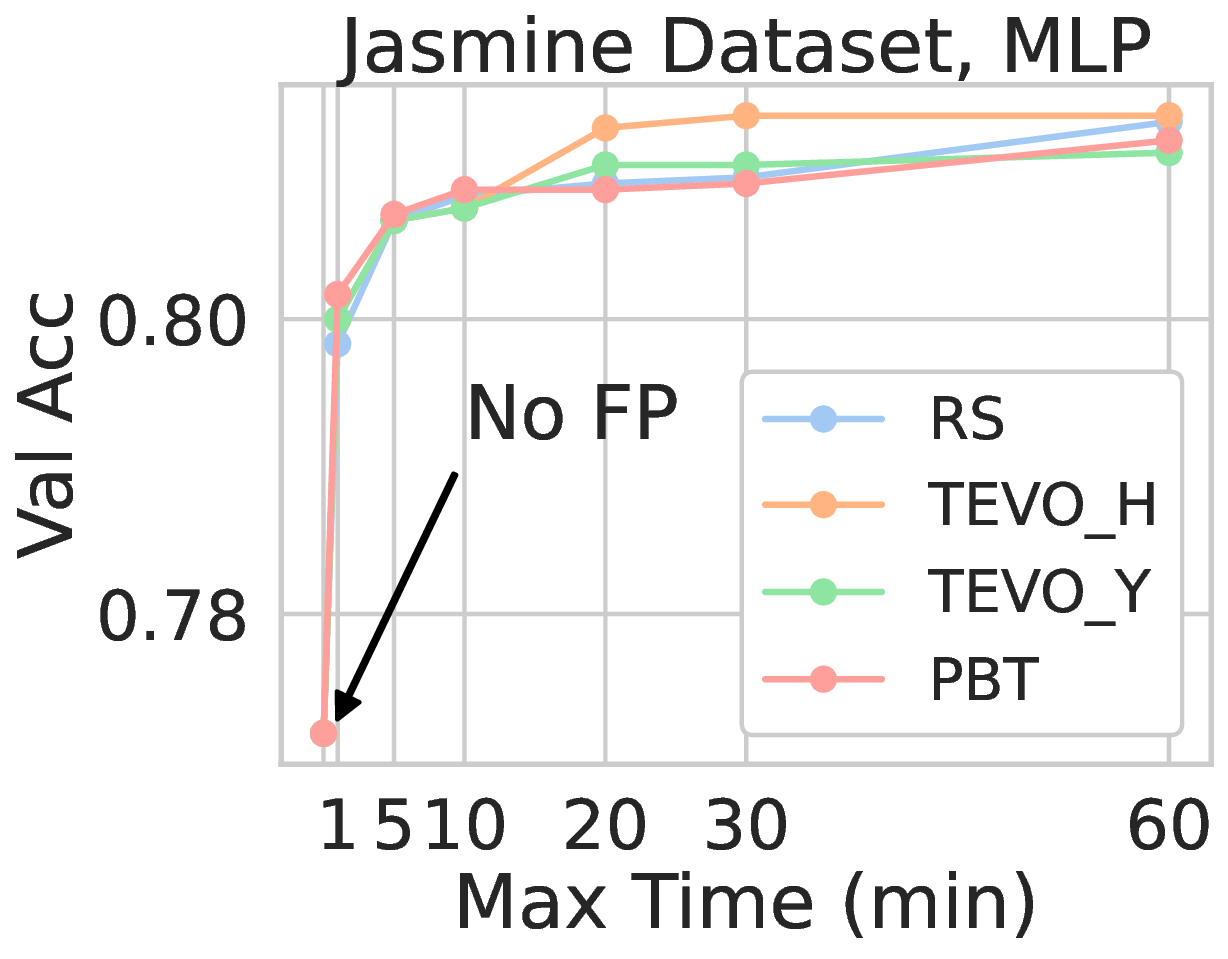}}
\subfigure[Madeline, MLP]{
\label{Fig.sub.2}
\includegraphics[width=0.18\textwidth]{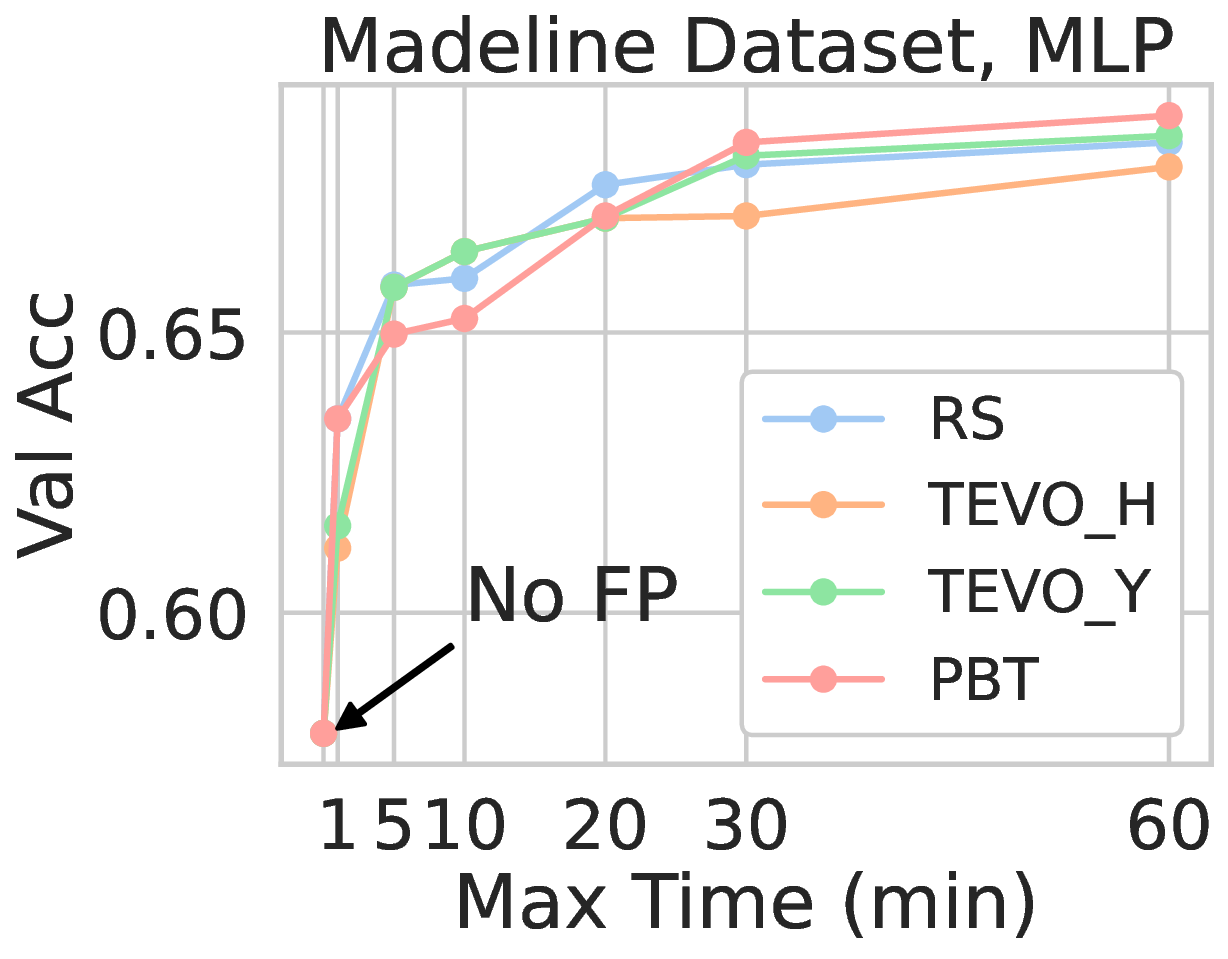}}
\subfigure[Pd\_speech\_features, MLP]{
\label{Fig.sub.3}
\includegraphics[width=0.18\textwidth]{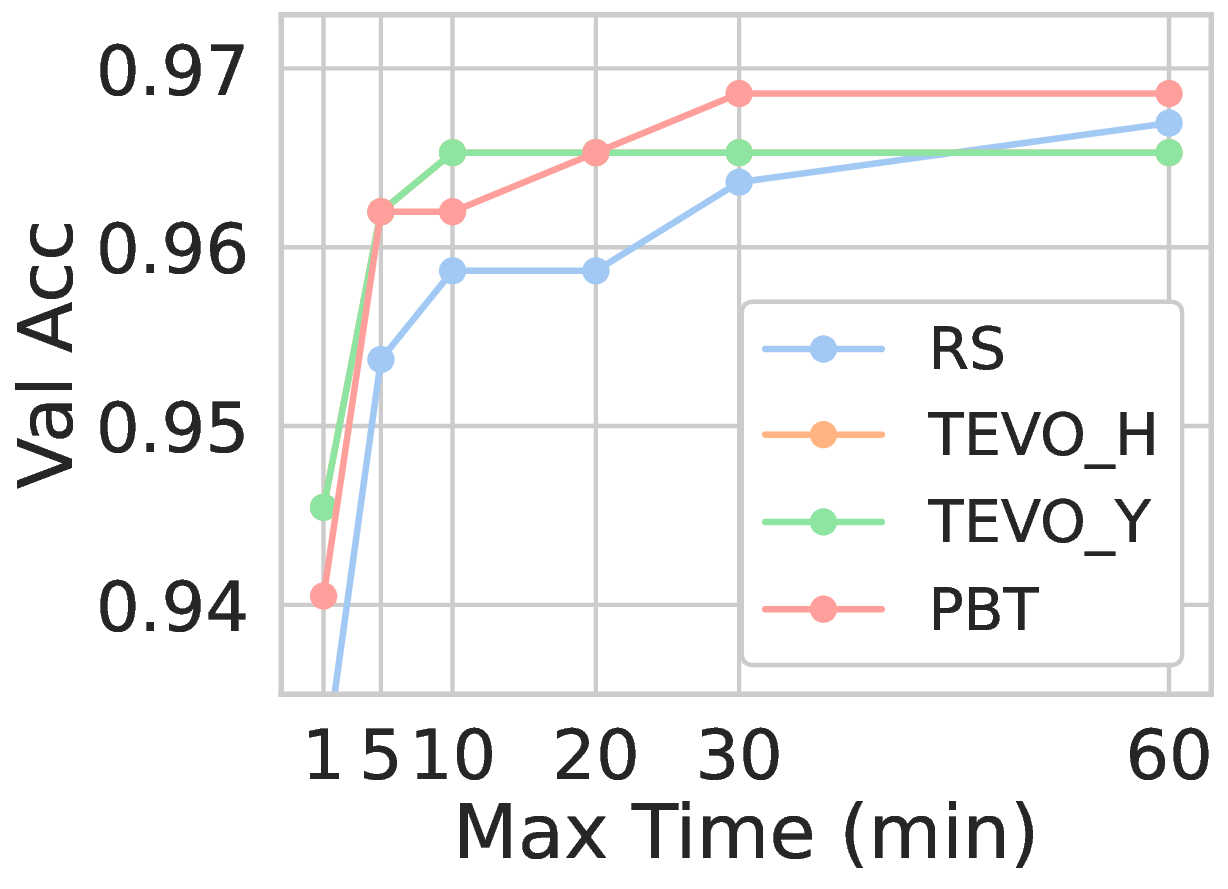}}
\subfigure[Wine\_quality, MLP]{
\label{Fig.sub.4}
\includegraphics[width=0.18\textwidth]{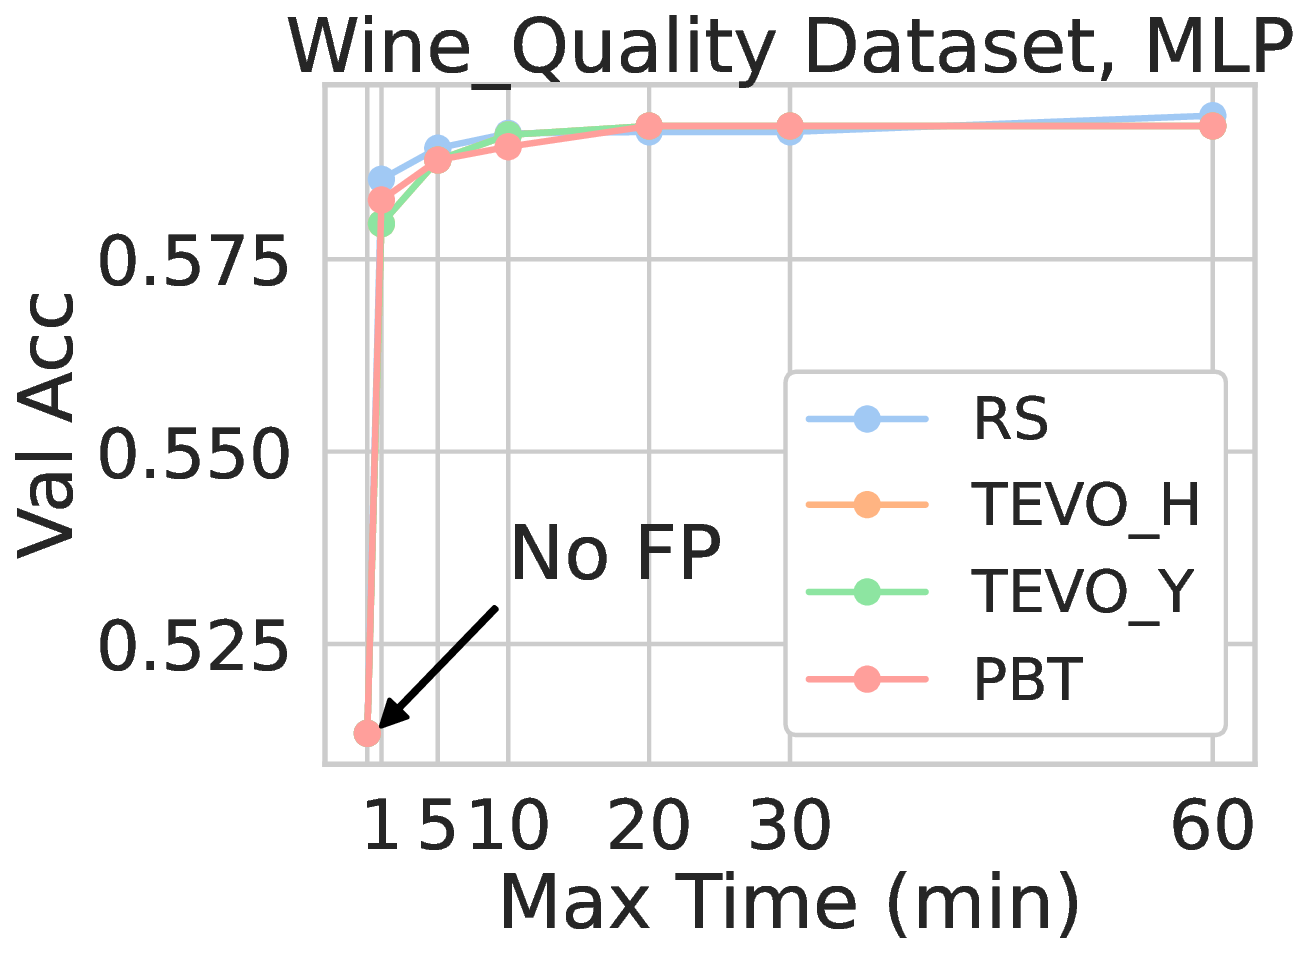}}
\subfigure[Thyroid\_allhyper, MLP]{
\label{Fig.sub.5}
\includegraphics[width=0.18\textwidth]{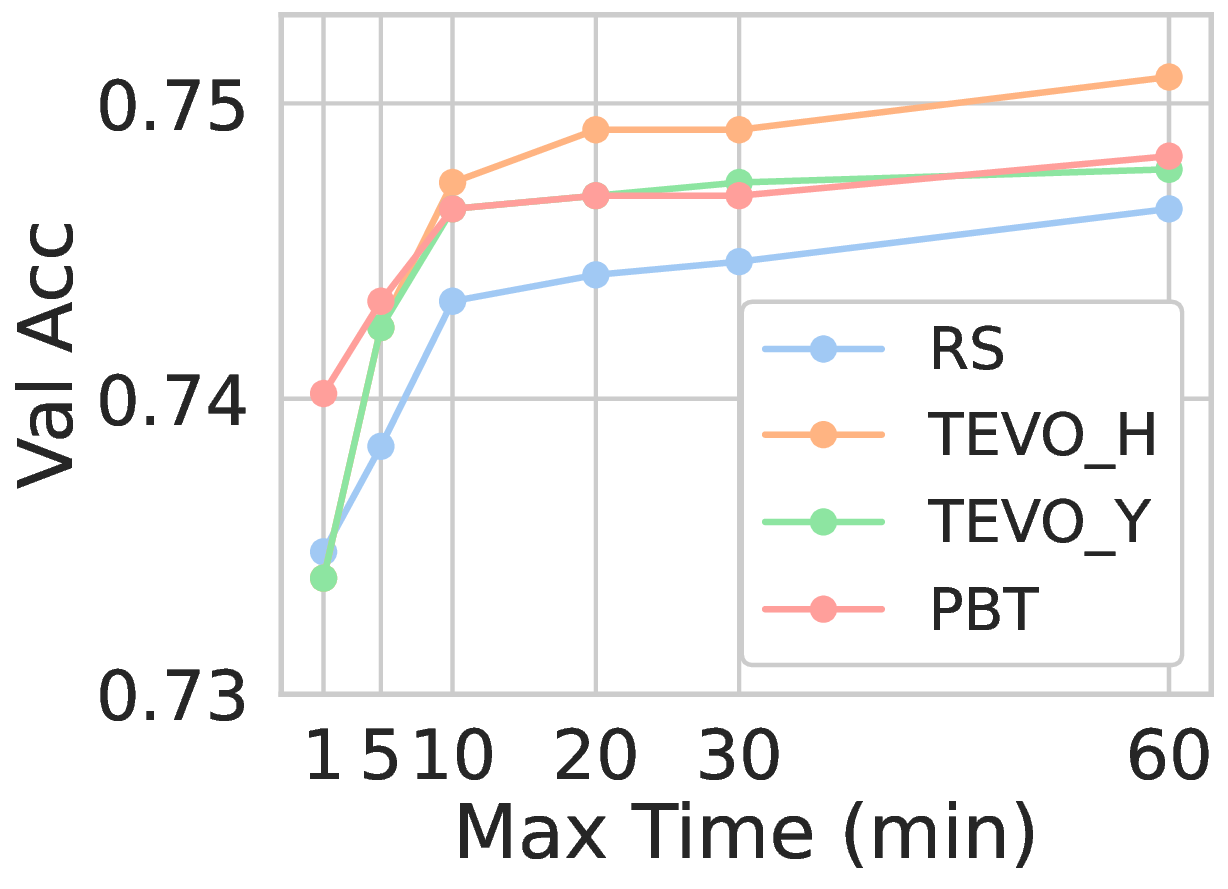}}
\caption{The trend of validation accuracy with the increasing of time limitation.}
\label{fig:max_scores_by_time}
\end{figure*}

\section{2}

\begin{figure*}[htbp]
\centering
\subfigure[Austrilian, LR]{
\label{Fig.sub.1}
\includegraphics[width=0.18\textwidth]{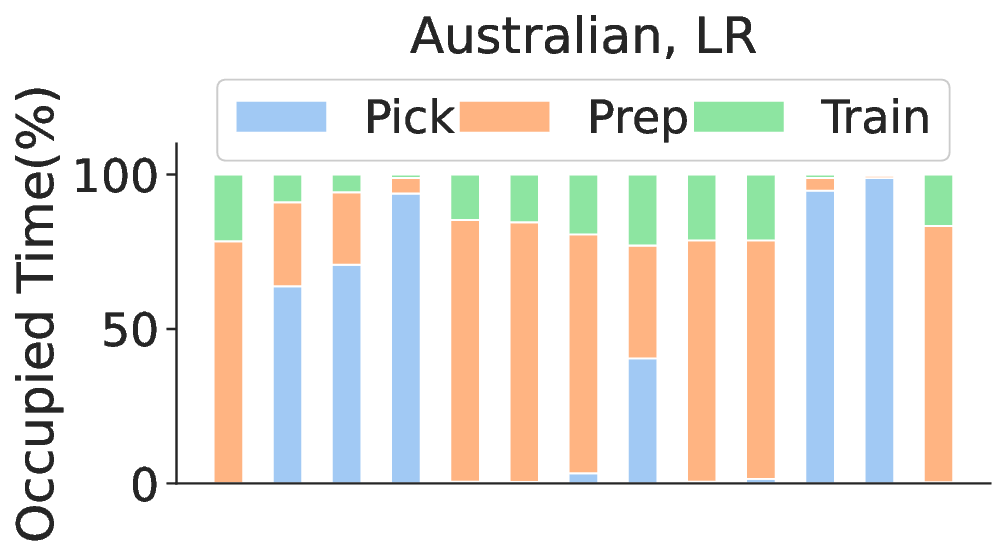}}
\subfigure[Blood, LR]{
\label{Fig.sub.2}
\includegraphics[width=0.18\textwidth]{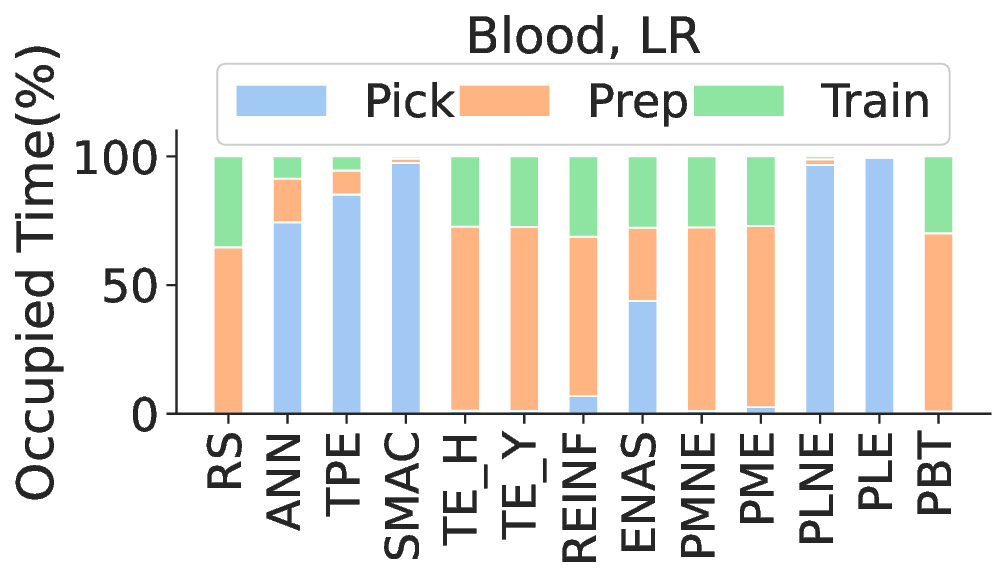}}
\subfigure[Emotion, LR]{
\label{Fig.sub.3}
\includegraphics[width=0.18\textwidth]{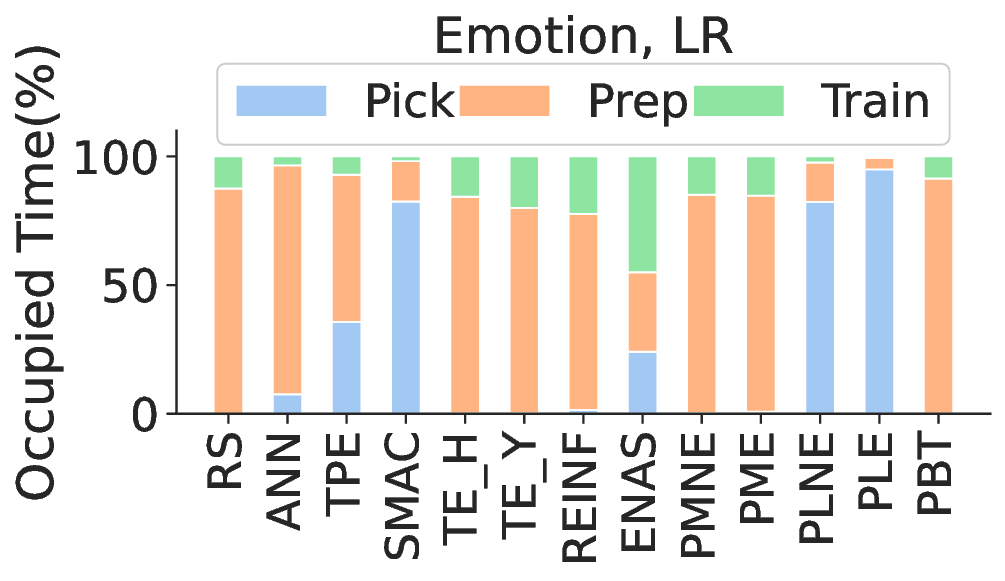}}
\subfigure[Heart, LR]{
\label{Fig.sub.4}
\includegraphics[width=0.18\textwidth]{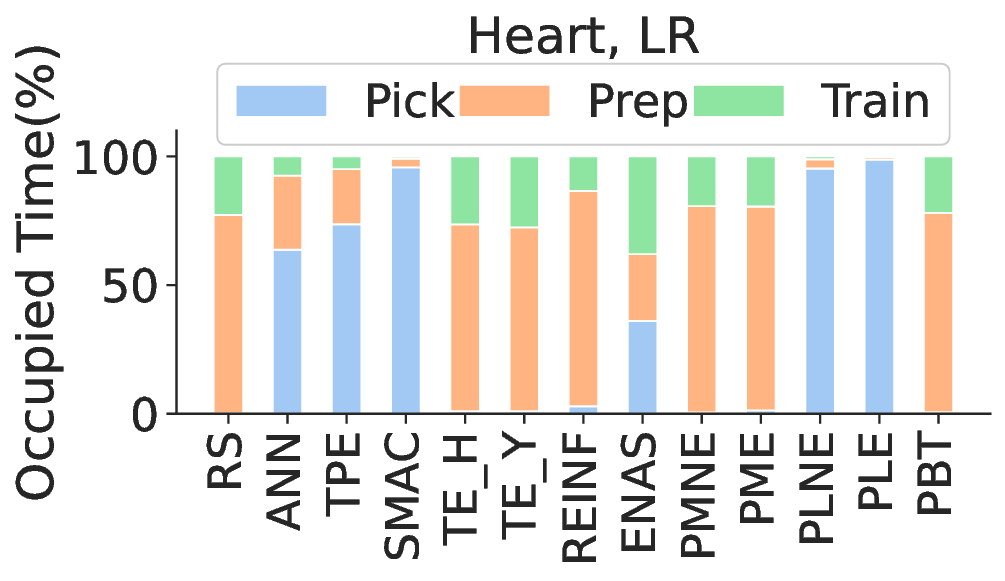}}
\subfigure[Forex, LR]{
\label{Fig.sub.5}
\includegraphics[width=0.18\textwidth]{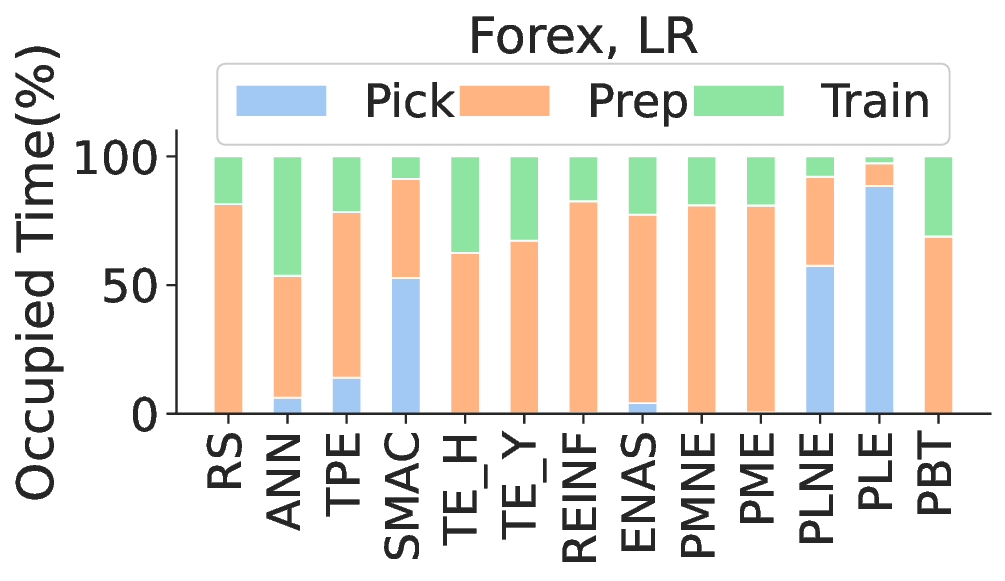}}
\subfigure[Jasmine, LR]{
\label{Fig.sub.6}
\includegraphics[width=0.18\textwidth]{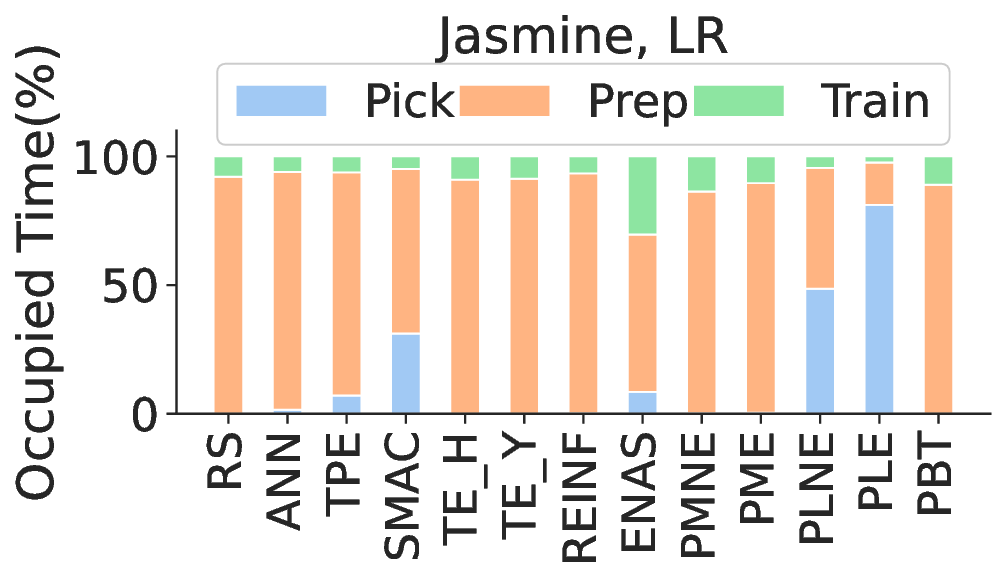}}
\subfigure[Madeline, LR]{
\label{Fig.sub.7}
\includegraphics[width=0.18\textwidth]{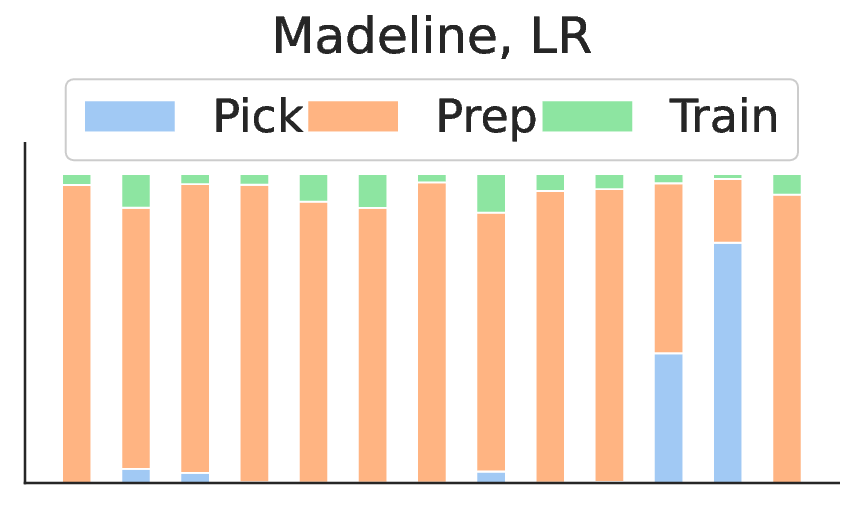}}
\subfigure[Pd\_speech\_features, LR]{
\label{Fig.sub.8}
\includegraphics[width=0.18\textwidth]{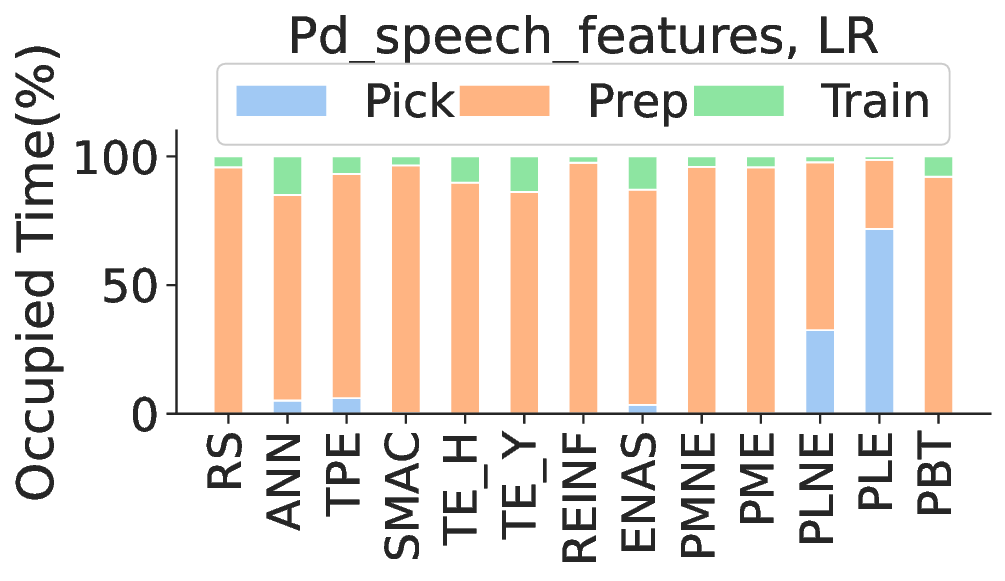}}
\subfigure[Wine\_quality, LR]{
\label{Fig.sub.9}
\includegraphics[width=0.18\textwidth]{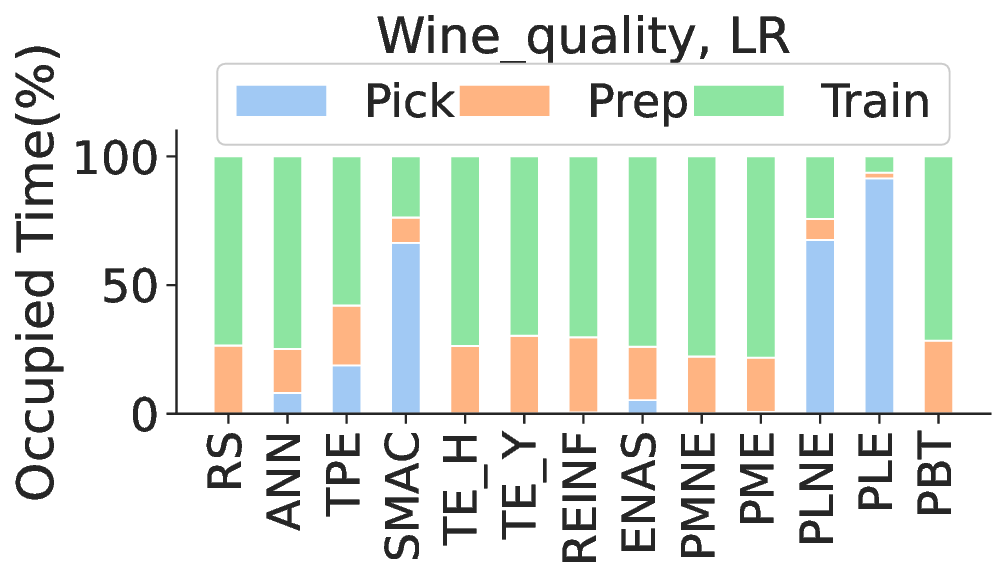}}
\subfigure[Thyroid\_allhyper, LR]{
\label{Fig.sub.10}
\includegraphics[width=0.18\textwidth]{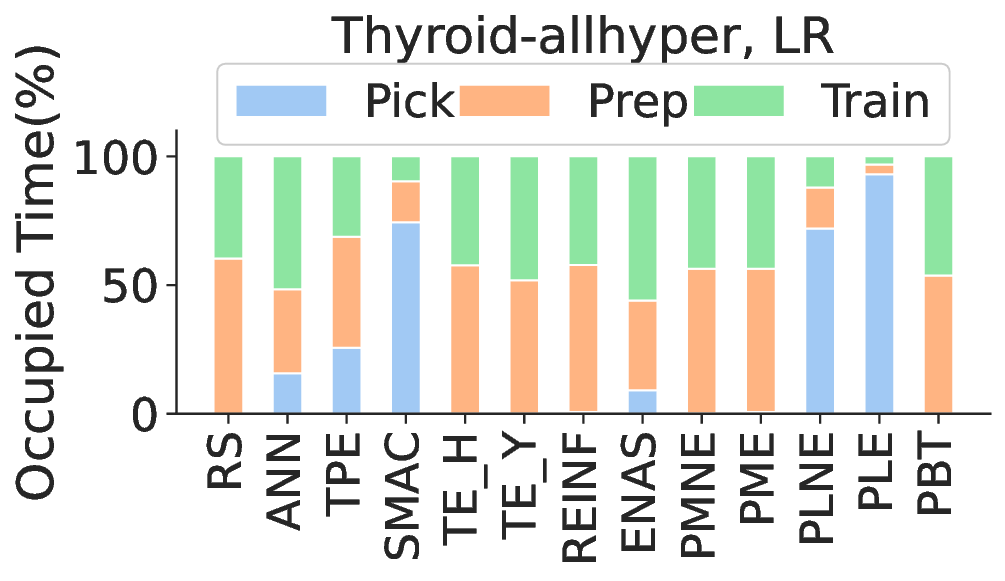}}
%\caption{Overhead of each calculating part on different dataset with downstream LR model.}
%\label{fig:overhead_LR}
%\end{figure*}

%\begin{figure*}[htbp]
%\centering
\subfigure[Austrilian, XGB]{
\label{Fig.sub.1}
\includegraphics[width=0.18\textwidth]{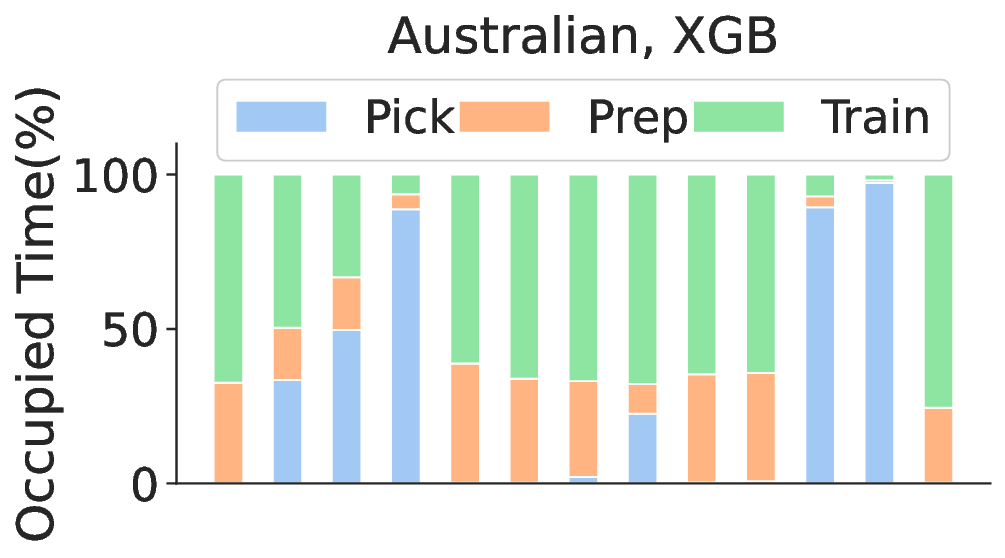}}
\subfigure[Blood, XGB]{
\label{Fig.sub.2}
\includegraphics[width=0.18\textwidth]{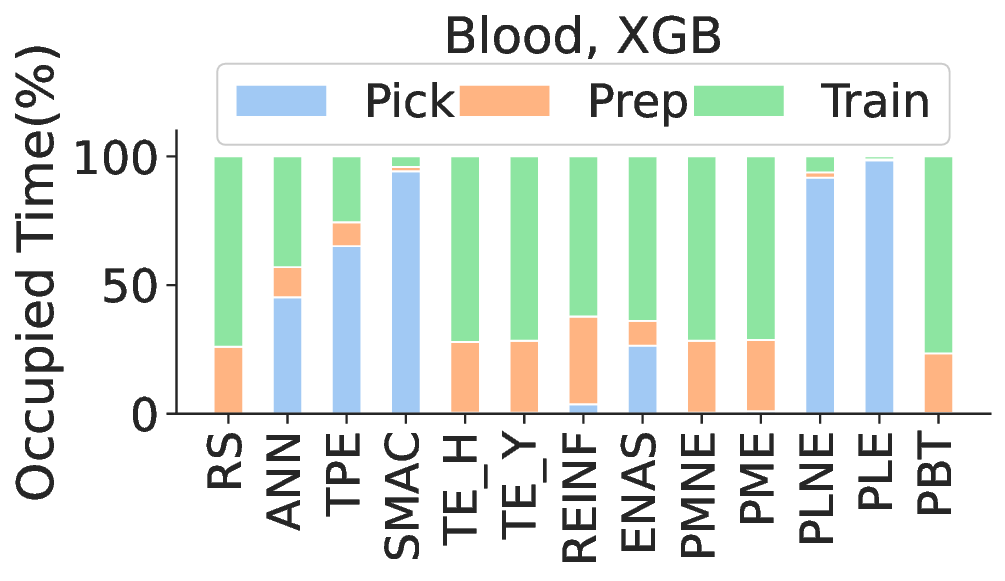}}
\subfigure[Emotion, XGB]{
\label{Fig.sub.3}
\includegraphics[width=0.18\textwidth]{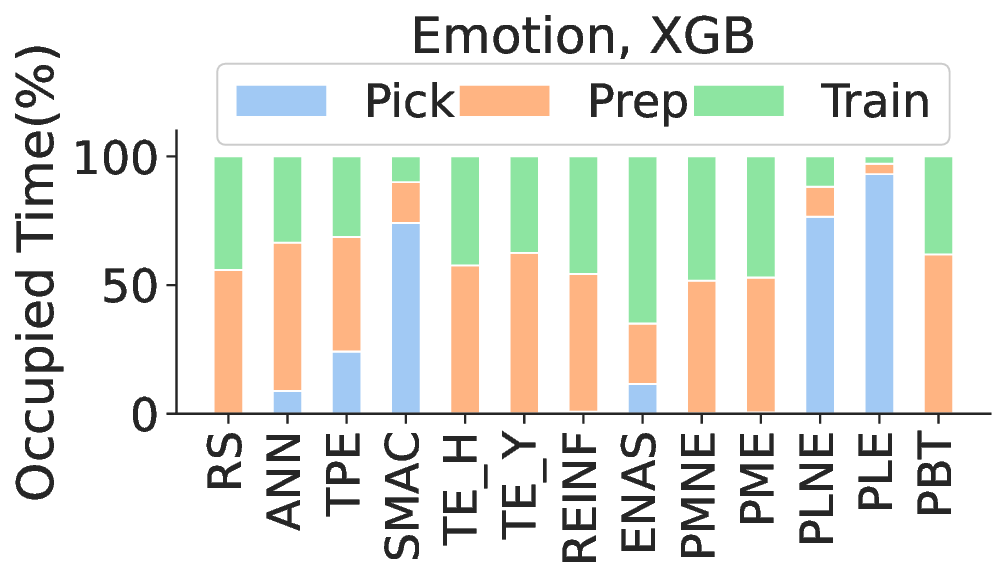}}
\subfigure[Heart, XGB]{
\label{Fig.sub.4}
\includegraphics[width=0.18\textwidth]{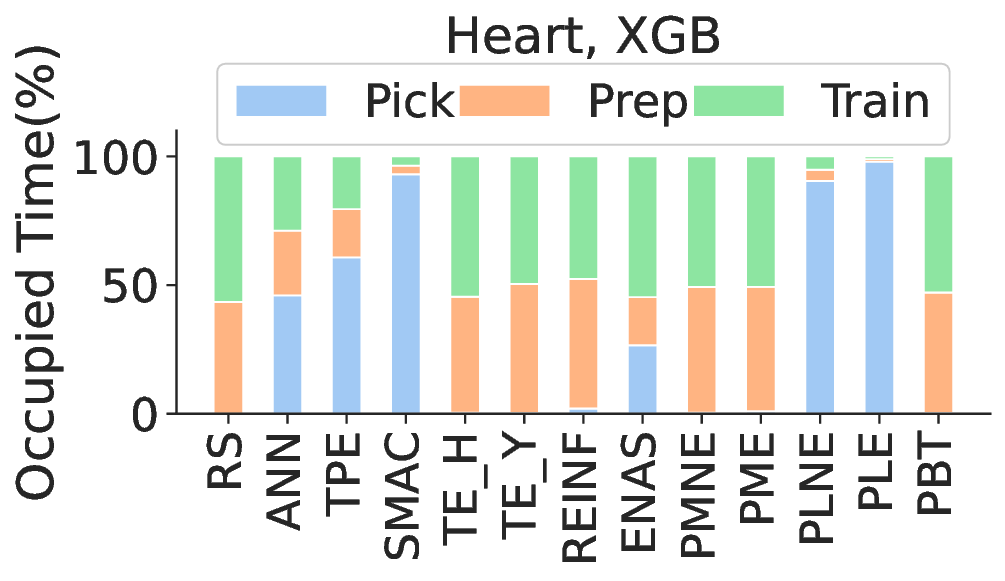}}
\subfigure[Forex, XGB]{
\label{Fig.sub.5}
\includegraphics[width=0.18\textwidth]{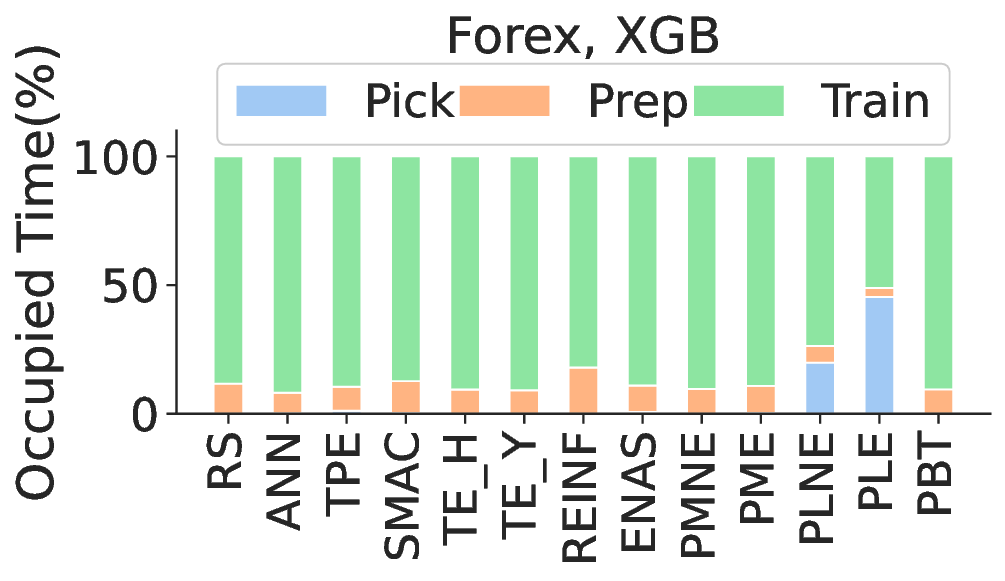}}
\subfigure[Jasmine, XGB]{
\label{Fig.sub.6}
\includegraphics[width=0.18\textwidth]{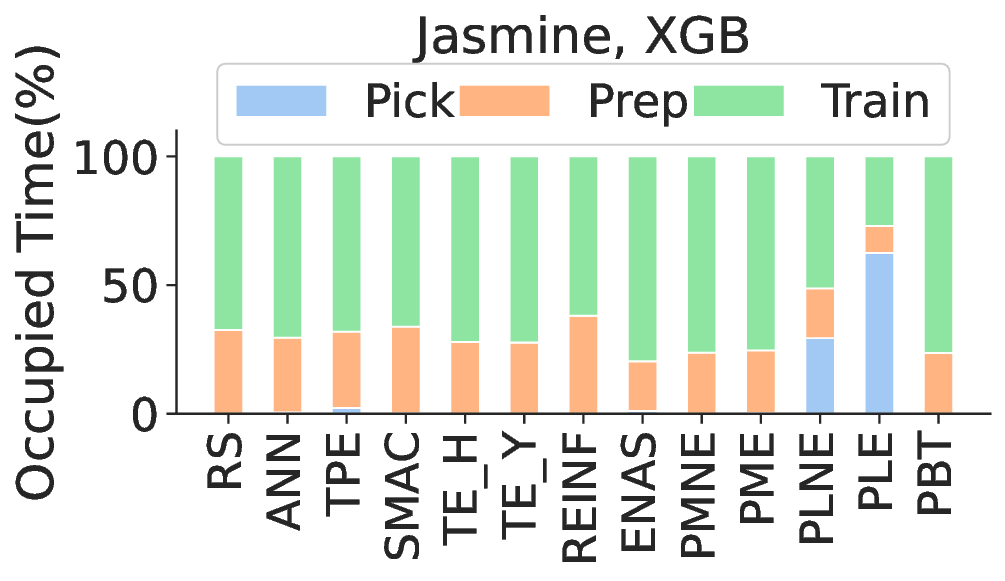}}
\subfigure[Madeline, XGB]{
\label{Fig.sub.7}
\includegraphics[width=0.18\textwidth]{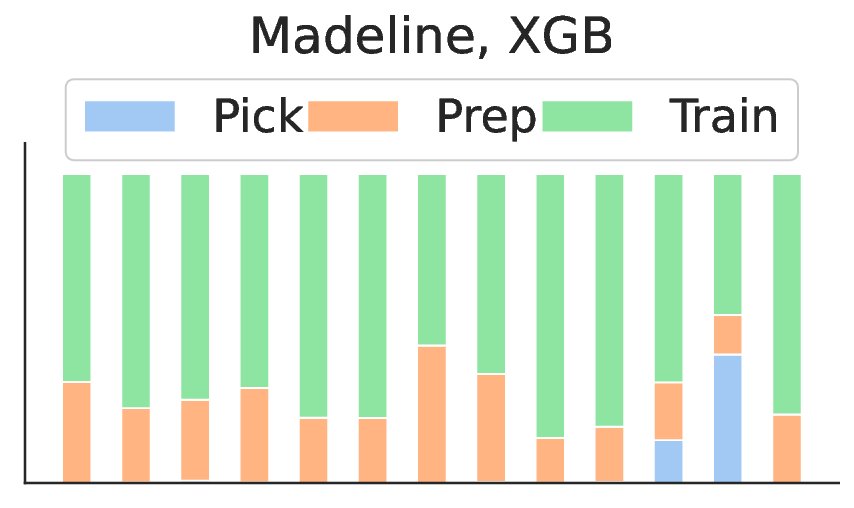}}
\subfigure[Pd\_speech\_features, XGB]{
\label{Fig.sub.8}
\includegraphics[width=0.18\textwidth]{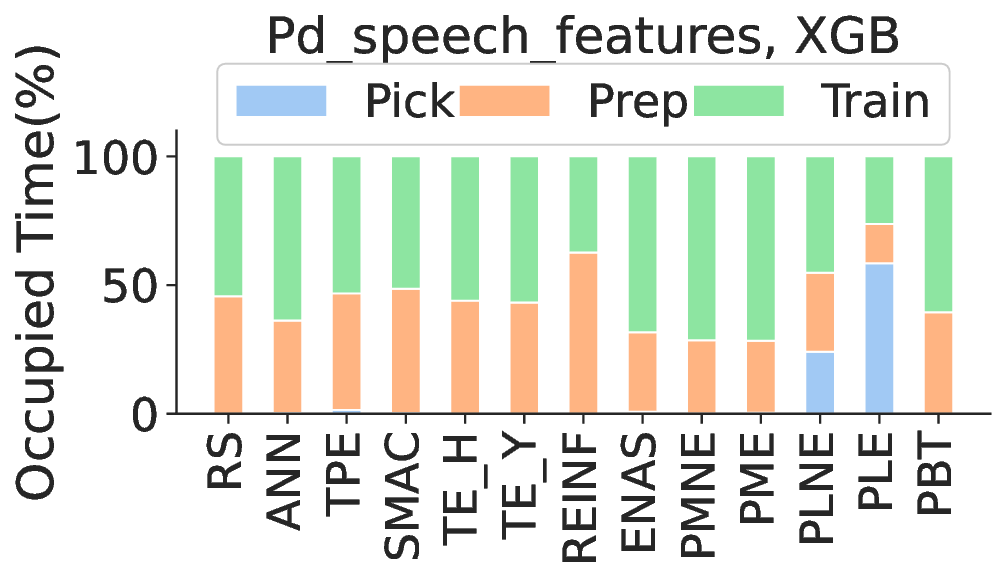}}
\subfigure[Wine\_quality, XGB]{
\label{Fig.sub.9}
\includegraphics[width=0.18\textwidth]{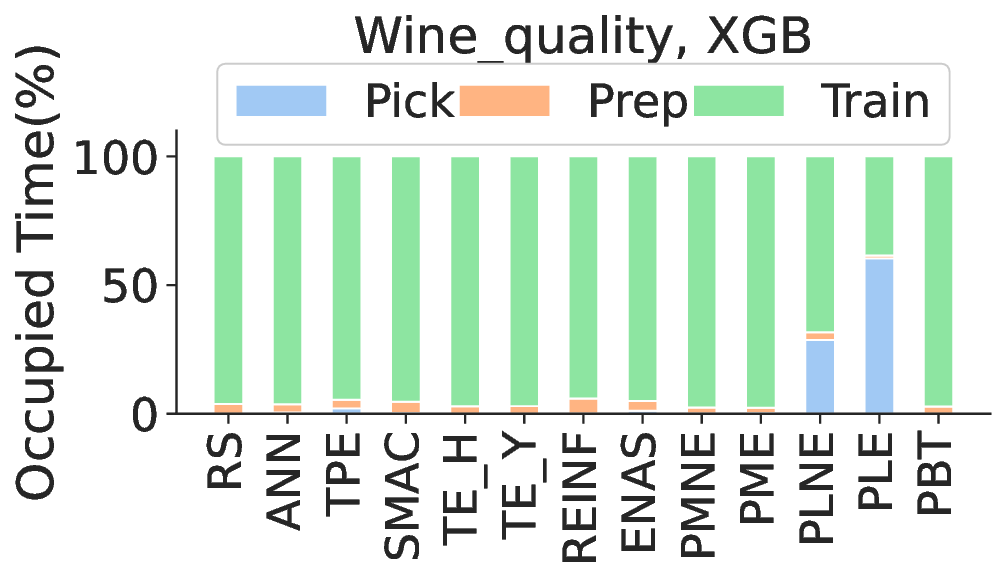}}
\subfigure[Thyroid\_allhyper, XGB]{
\label{Fig.sub.10}
\includegraphics[width=0.18\textwidth]{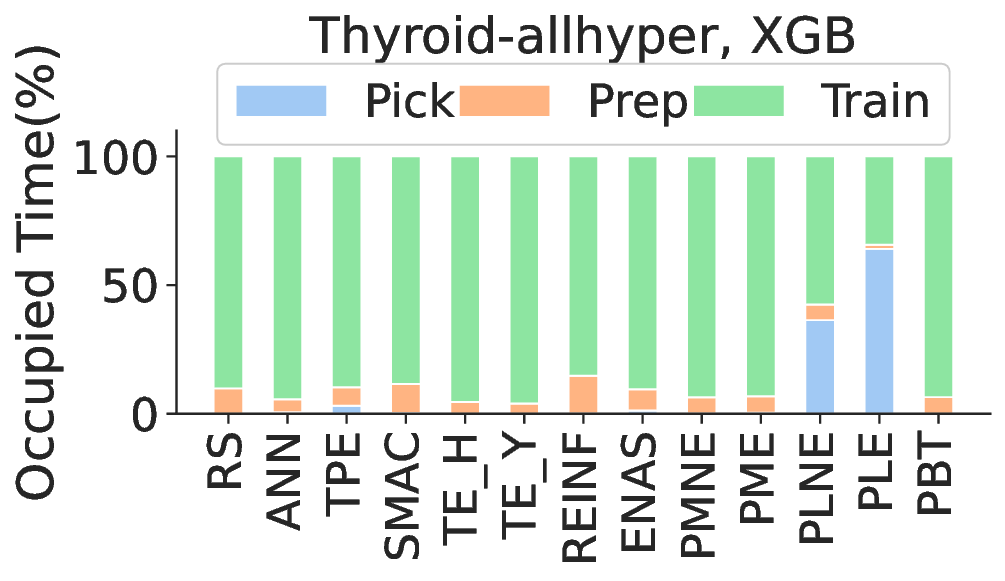}}
%\caption{Overhead of each calculating part on different dataset with downstream XGB model.}
%\label{fig:overhead_XGB}
%\end{figure*}

%\begin{figure*}[htbp]
%\centering
\subfigure[Austrilian, MLP]{
\label{Fig.sub.1}
\includegraphics[width=0.18\textwidth]{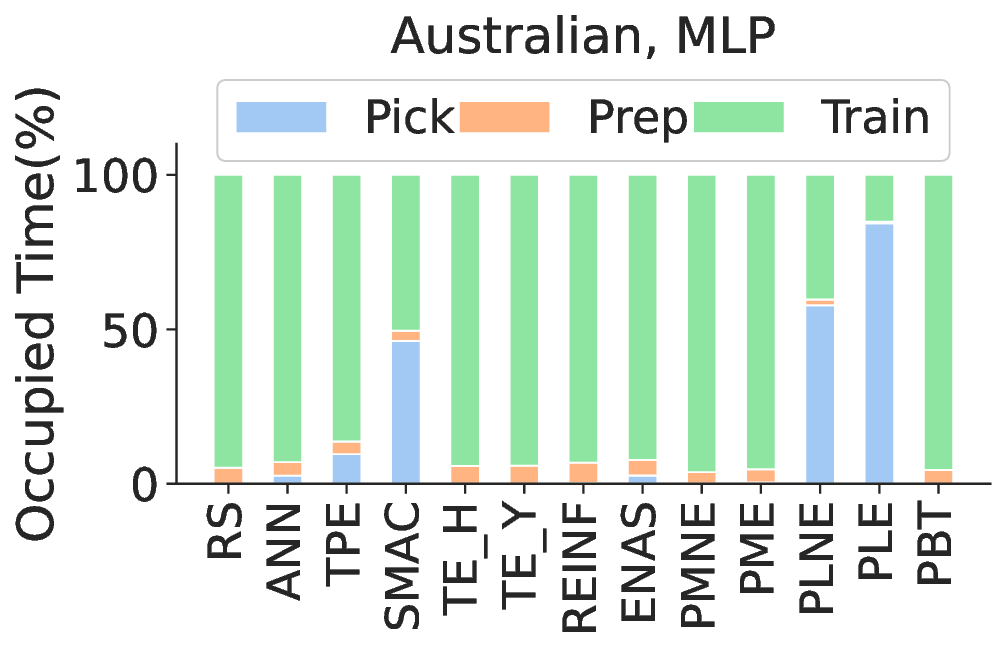}}
\subfigure[Blood, MLP]{
\label{Fig.sub.2}
\includegraphics[width=0.18\textwidth]{figures/overhead_blood_XGB_600.eps}}
\subfigure[Emotion, MLP]{
\label{Fig.sub.3}
\includegraphics[width=0.18\textwidth]{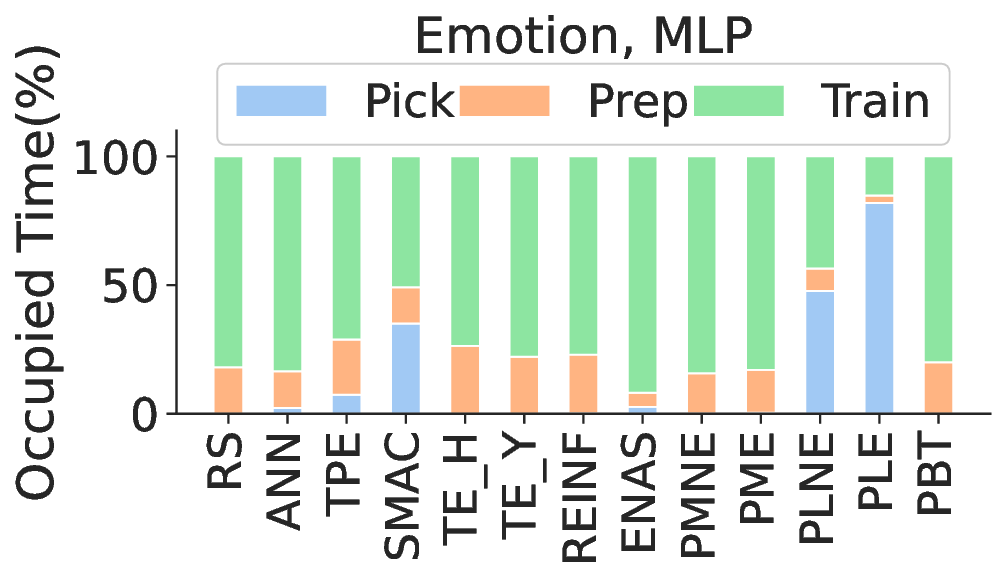}}
\subfigure[Heart, MLP]{
\label{Fig.sub.4}
\includegraphics[width=0.18\textwidth]{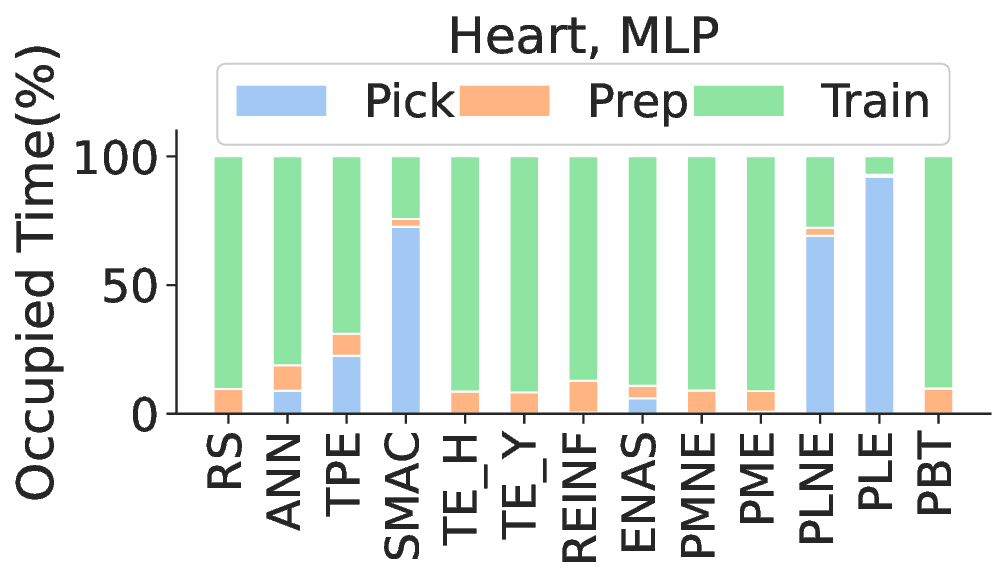}}
\subfigure[Forex, MLP]{
\label{Fig.sub.5}
\includegraphics[width=0.18\textwidth]{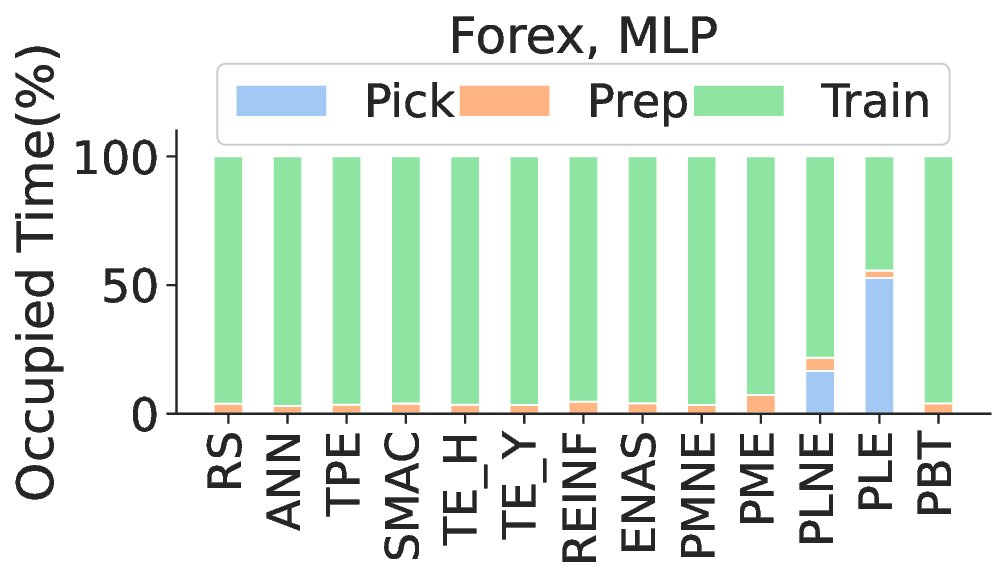}}
\subfigure[Jasmine, MLP]{
\label{Fig.sub.6}
\includegraphics[width=0.18\textwidth]{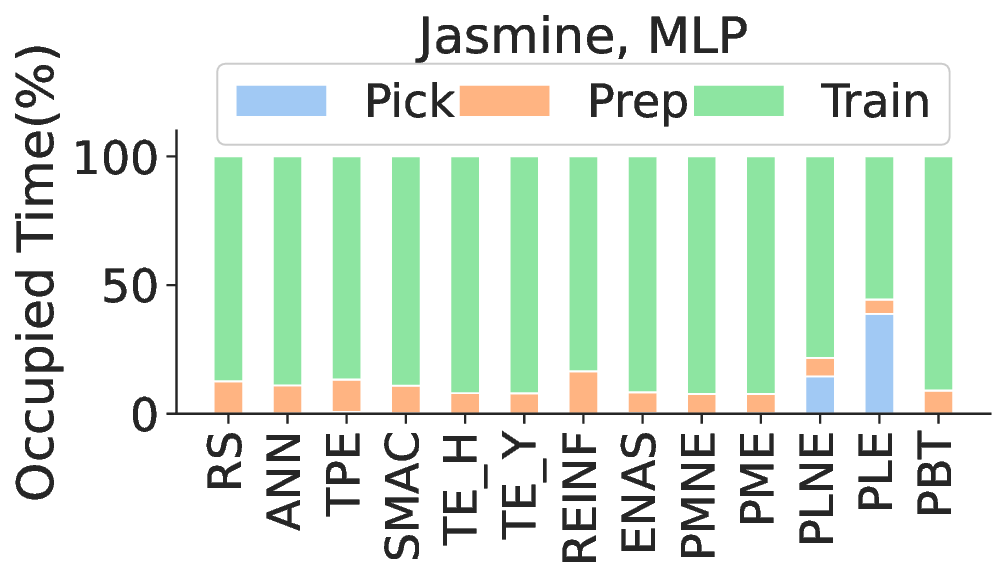}}
\subfigure[Madeline, MLP]{
\label{Fig.sub.7}
\includegraphics[width=0.18\textwidth]{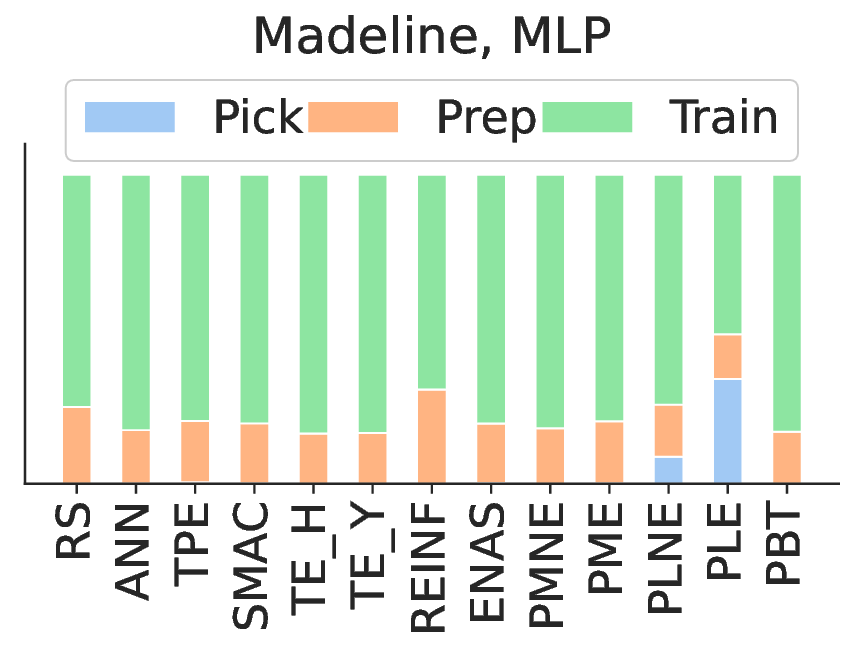}}
\subfigure[Pd\_speech\_features, MLP]{
\label{Fig.sub.8}
\includegraphics[width=0.18\textwidth]{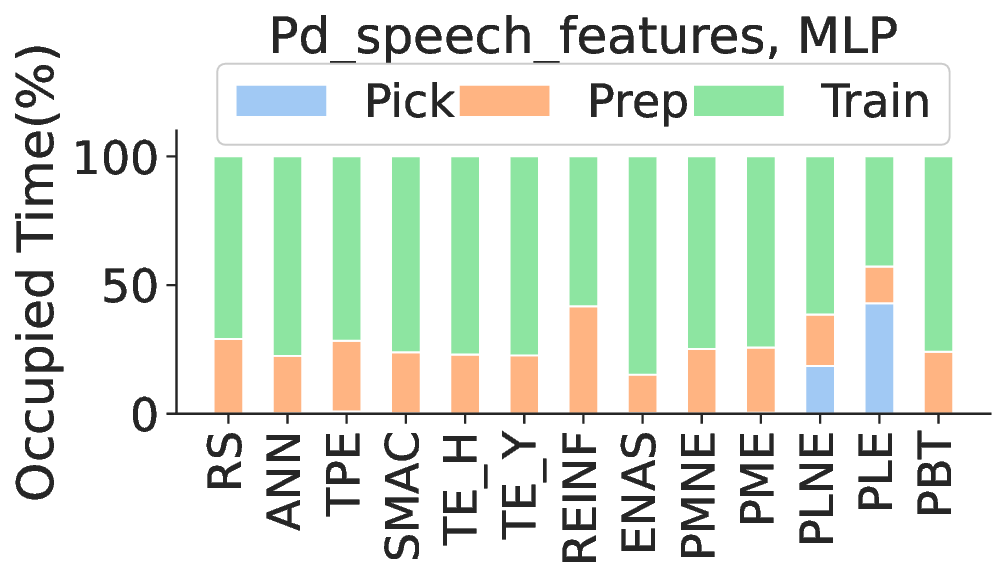}}
\subfigure[Wine\_quality, MLP]{
\label{Fig.sub.9}
\includegraphics[width=0.18\textwidth]{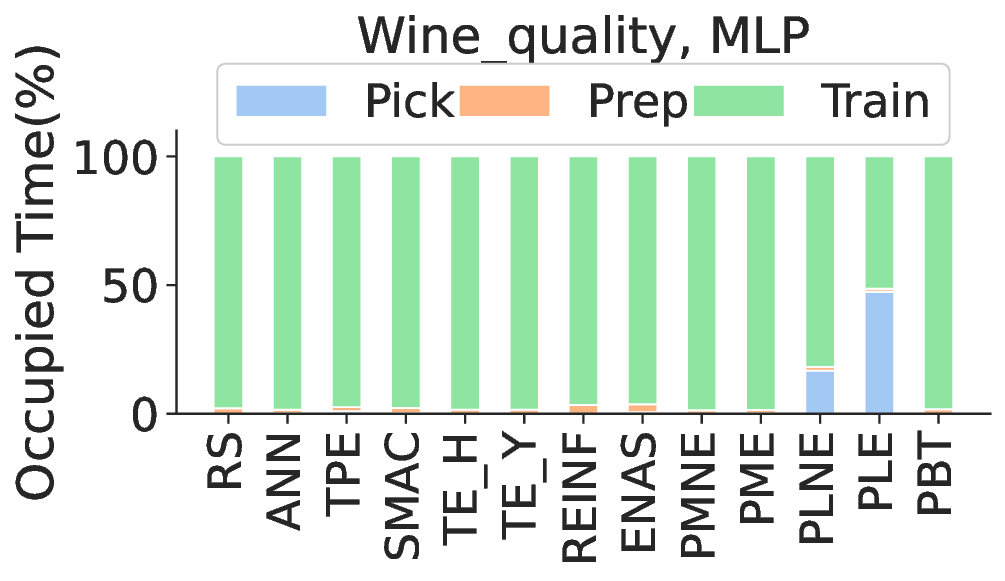}}
\subfigure[Thyroid\_allhyper, MLP]{
\label{Fig.sub.10}
\includegraphics[width=0.18\textwidth]{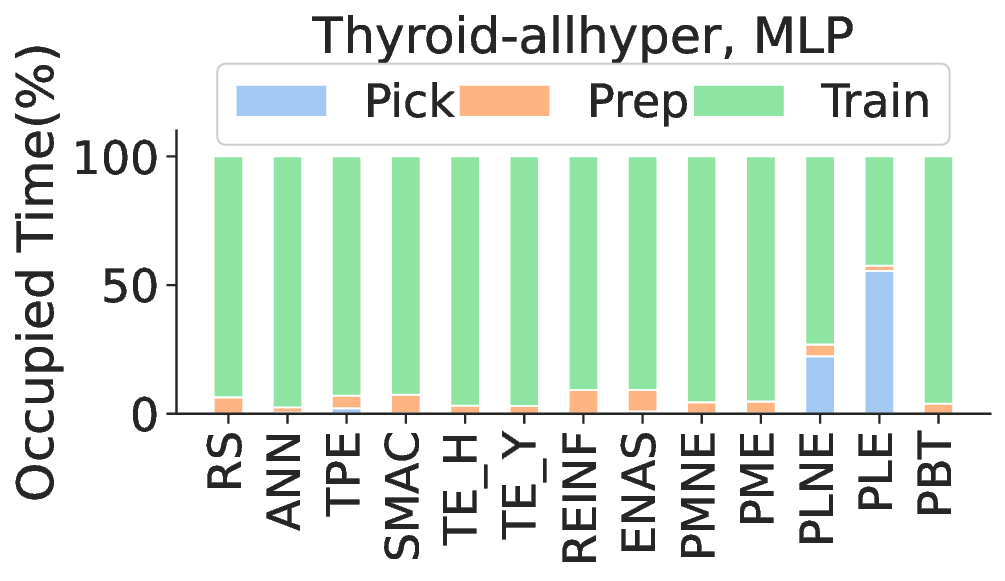}}
\caption{Overhead of each calculating part on different dataset with different downstream ML models.}
\label{fig:overhead}
\end{figure*}

\section{3}
\begin{table*}[t]% h asks to places the floating element [h]ere.
  \caption{$\Delta \  Acc$ on 10 datasets under 60 seconds time constrain.}
  \label{tab:delta_acc_60_appendix1}
  \footnotesize
  \begin{tabular}{p{0.06\textwidth}<{\centering}|
                  p{0.034\textwidth}<{\centering}|
                  p{0.03\textwidth}<{\centering}
                  p{0.034\textwidth}<{\centering}|
                  p{0.03\textwidth}<{\centering}
                  p{0.034\textwidth}<{\centering}|
                  p{0.04\textwidth}<{\centering}
                  p{0.04\textwidth}<{\centering}
                  p{0.032\textwidth}<{\centering}|
                  p{0.054\textwidth}<{\centering}
                  p{0.034\textwidth}<{\centering}|
                  p{0.06\textwidth}<{\centering}
                  p{0.035\textwidth}<{\centering}|
                  p{0.03\textwidth}<{\centering}
                  p{0.03\textwidth}<{\centering}
                  p{0.03\textwidth}<{\centering}
                  p{0.035\textwidth}<{\centering}}
    \toprule
    Dataset & ML Model & RS & Anneal & TPE & SMAC & TEVO\_H & TEVO\_Y & PBT & REINFORCE & ENAS & HYPERBAND & BOHB & PMNE & PME & PLNE & PLE \\
    \midrule
               & LR & \textbf{+3.07} & +1.81 & +1.81 & +1.81 & +2.35 & +2.71 & +2.53 & +2.89 & +2.35 & +1.99 & +1.45 & +1.99 & +1.99 & +1.27 & +0.91\\
    Austrilian & XGB & +3.21 & +2.49 & +2.85 & +2.85 & \textbf{+3.75} & +3.93 & \textbf{+3.75} & +2.85 & +1.59 & +2.67 & +0.51 & +2.85 & +2.85 & +1.05 & +0.00\\
               & MLP & +5.15 & +4.97 & +4.43 & +3.89 & \textbf{+5.69} & \textbf{+5.69} & +5.15 & +4.07 & +3.53 & +3.89 & +3.89 & +4.07 & +4.07 & +4.43 & +3.89\\
    \midrule
          & LR & +3.50 & +3.33 & +3.33 & +3.33 & +4.00 & +4.00 & \textbf{+4.17} & +2.83 & +1.67 & +3.50 & +2.33 & +3.33 & +3.33 & +3.33 & +3.33 \\
    Blood & XGB & +8.29 & +6.95 & +7.79 & +6.95 & +8.95 & +8.79 & \textbf{+9.95} & +8.45 & +7.62 & +8.29 & +7.62 & +8.62 & +8.62 & +6.79 & +5.62\\
          & MLP & +6.78 & +6.78 & +6.61 & \textbf{+7.28} & +6.95 & +6.95 & \textbf{+7.28} & +5.45 & +5.61 & +6.45 & +6.45 & \textbf{+7.28} & \textbf{+7.28} & +6.45 & +6.45\\
    \midrule
            & LR & +10.16 & +9.21 & +8.26 & +9.53 & +9.21 & +8.58 & +10.48 & \textbf{+11.12} & +8.58 & +8.26 & +6.99 & +7.62 & +7.62 & +7.94 & +6.35\\
    Emotion & XGB & +0.42 & +0.1 & +0.42 & +0.74 & +1.05 & +0.42 & +0.42 & \textbf{+1.37} & +0.00 & +0.10 & +0.00 & +0.00 & +0.00 & +0.00 & +0.00\\
            & MLP & +44.23 & +43.92 & \textbf{+44.55} & +43.60 & +43.92 & +43.92 & +43.92 & +42.96 & +43.28 & +42.96 & +43.60 & +43.92 & +43.6 & +44.23 & +41.69\\
    \midrule
          & LR & +13.50 & \textbf{+16.32} & +14.79 & +12.97 & +14.67 & +14.15 & +13.12 & +10.87 & +10.73 & +0.00 & +0.00 & +11.94 & +11.16 & +10.00 & +9.98\\
    Forex & XGB & +5.79 & +5.85 & +3.60 & +3.73 & +4.85 & +4.85 & \textbf{+9.32} & +0.00 & +0.00 & +0.00 & +0.00 & +0.09 & +0.09 & +2.27 & +0.09\\
          & MLP & +7.93 & +3.23 & +3.28 & +0.72 & +5.76 & +5.76 & \textbf{+7.24} & +0.00 & +0.00 & +0.00 & +0.00 & +0.81 & +0.81 & +0.78 & +0.78\\
    \midrule
          & LR & +6.12 & +4.08 & +4.49 & +6.12 & \textbf{+7.35} & \textbf{+7.35} & +5.31 & +5.72 & +4.08 & +4.49 & +3.27 & +6.12 & +6.12 & +2.45 & +0.41\\
    Heart & XGB & +3.84 & +0.16 & +0.16 & +2.20 & +2.61 & +3.02 & \textbf{+3.84} & +0.98 & +0.00 & +0.57 & +0.00 & +2.20 & +2.20 & +0.00 & +0.00\\
          & MLP & +26.94 & +26.13 & +27.76 & +26.53 & +27.76 & +27.76 & +27.35 & \textbf{+28.17} & +25.31 & +25.72 & +24.90 & +25.31 & +26.13 & +26.13 & +24.49\\
    \midrule
            & LR & +2.85 & +2.94 & +2.89 & +2.73 & +2.89 & +2.89 & +2.85 & \textbf{+3.02} & +2.98 & +0.00 & +0.00 & +2.73 & +2.73 & +2.81 & +2.73\\
    Jasmine & XGB & +1.34 & +1.09 & +1.25 & +0.92 & \textbf{+1.38} & \textbf{+1.38} & +1.30 & +0.33 & +0.38 & +0.00 & +0.00 & +1.09 & +1.30 & +1.09 & +1.00\\
            & MLP & +1.73 & +1.69 & +2.32 & +2.23 & +1.90 & +1.90 & +2.07 & +1.23 & +1.82 & +0.00 & +0.00 & \textbf{+2.23} & \textbf{+2.23} & \textbf{+2.23} & \textbf{+2.23}\\
    \midrule
             & LR & +4.86 & +5.17 & +4.86 & +2.99 & \textbf{+5.49} & \textbf{+5.49} & +5.29 & +3.66 & +3.15 & +0.00 & +0.00 & +4.98 & +4.98 & +4.06 & +3.39\\
    Madeline& XGB & +0.10 & +0.00 & +0.00 & +0.00 & +0.00 & +0.00 & +0.14 & +0.00 & +0.00 & +0.00 & +0.00 & \textbf{+0.62} & \textbf{+0.62} & \textbf{+0.62} & \textbf{+0.62}\\
             & MLP & +12.30 & +11.46 & +11.78 & +13.25 & +9.99 & +10.39 & +12.30 & +8.52 & +7.37 & +0.00 & +0.00 & +13.85 & +13.85 & \textbf{+14.13} & +13.85\\
    \midrule
                         & LR & +11.14 & +10.98 & +11.14 & +11.8 & +11.31 & +11.64 & \textbf{+11.97} & +1.55 & +6.18 & +0.00 & +0.00 & +11.80 & +11.80 & +11.80 & +11.80\\
    \makecell{Pd\_speech\\ \_features} & XGB & +2.37 & +2.70 & +2.37 & +1.88 & +2.37 & +2.37 & \textbf{+3.03} & +0.00 & +0.00 & +0.00 & +0.00 & +2.21 & +1.88 & +1.88 & +2.37\\
                         & MLP & +19.94 & +19.44 & +21.09 & +19.44 & +21.43 & +21.43 & +20.93 & +6.88 & +15.48 & +0.00 & +0.00 & +21.92 & +21.92 & \textbf{+22.25} & \textbf{+22.25}\\
    \midrule
                  & LR & +8.38 & +8.37 & +8.25 & \textbf{+9.13} & +8.04 & +8.42 & +8.13 & +8.46 & +6.52 & +8.38 & +8.17 & +7.96 & +7.94 & +8.29 & +7.88\\
    \makecell{Wine\\ \_quality} & XGB & +0.00 & +0.00 & +0.00 & +0.00 & +0.00 & +0.00 & +0.00 & +0.00 & +0.00 & +0.00 & +0.00 & +0.00 & +0.00 & +0.00 & +0.00\\
                  & MLP & +7.75 & +4.92 & +7.13 & \textbf{+8.15} & +7.17 & +7.17 & +7.48 & +0.00 & +0.92 & +0.00 & +0.00 & \textbf{+8.15} & \textbf{+8.15} & \textbf{+8.15} & \textbf{+8.15}\\
    \midrule
                      & LR & +6.70 & +6.56 & +6.88 & +6.03 & +7.05 & +7.05 & \textbf{+7.28} & +6.07 & +5.80 & +6.56 & +6.12 & +6.92 & +6.65 & +6.07 & +6.03\\
    \makecell{Thyroid\\ \_allhyper} & XGB & +1.09 & +1.58 & +2.21 & \textbf{+2.88} & +2.38 & +2.38 & +2.43 & +0.00 & +0.00 & +0.51 & +0.42 & +1.27 & +1.18 & +1.63 & +0.64\\
                      & MLP & +4.91 & +4.60 & +4.73 & \textbf{+5.76} & +4.82 & +4.82 & +5.45 & +1.47 & +2.23 & +0.00 & +0.00 & +5.09 & +5.09 & +5.09 & +5.09\\
  \bottomrule
\end{tabular}
\end{table*}

\begin{table*}[htbp]% h asks to places the floating element [h]ere.
  \caption{Ranking on 10 datasets under 60 seconds time constrain.}
  \label{tab:delta_acc_60_appendix}
  \footnotesize
  \begin{tabular}{p{0.06\textwidth}<{\centering}|
                  p{0.034\textwidth}<{\centering}|
                  p{0.03\textwidth}<{\centering}
                  p{0.034\textwidth}<{\centering}|
                  p{0.03\textwidth}<{\centering}
                  p{0.034\textwidth}<{\centering}|
                  p{0.04\textwidth}<{\centering}
                  p{0.04\textwidth}<{\centering}
                  p{0.032\textwidth}<{\centering}|
                  p{0.054\textwidth}<{\centering}
                  p{0.034\textwidth}<{\centering}|
                  p{0.06\textwidth}<{\centering}
                  p{0.035\textwidth}<{\centering}|
                  p{0.03\textwidth}<{\centering}
                  p{0.03\textwidth}<{\centering}
                  p{0.03\textwidth}<{\centering}
                  p{0.035\textwidth}<{\centering}}
    \toprule
    Dataset & ML Model & RS & Anneal & TPE & SMAC & TEVO\_H & TEVO\_Y & PBT & REINFORCE & ENAS & HYPERBAND & BOHB & PMNE & PME & PLNE & PLE \\
    \midrule
               & LR & 1 & 10 & 12 & 11 & 5 & 3 & 4 & 2 & 6 & 9 & 13 & 7 & 8 & 14 & 15\\
    Austrilian & XGB & 4 & 11 & 9 & 5 & 2 & 1 & 3 & 8 & 12 & 10 & 14 & 6 & 7 & 13 & 15\\
               & MLP & 3 & 5 & 7 & 12 & 1 & 2 & 4 & 10 & 15 & 13 & 14 & 8 & 9 & 6 & 11\\
    \midrule
          & LR & 4 & 10 & 12 & 11 & 3 & 2 & 1 & 13 & 15 & 5 & 14 & 8 & 6 & 9 & 7 \\
    Blood & XGB & 7 & 13 & 9 & 12 & 2 & 3 & 1 & 6 & 10 & 8 & 11 & 4 & 5 & 14 & 15\\
          & MLP & 7 & 8 & 9 & 3 & 5 & 6 & 4 & 15 & 14 & 12 & 13 & 1 & 2 & 11 & 10\\
    \midrule
            & LR & 3 & 5 & 9 & 4 & 6 & 8 & 2 & 1 & 7 & 10 & 14 & 12 & 13 & 14 & 10\\
    Emotion & XGB & 5 & 8 & 4 & 3 & 2 & 6 & 7 & 1 & 10 & 9 & 11 & 14 & 13 & 12 & 15\\
            & MLP & 3 & 4 & 1 & 11 & 6 & 7 & 5 & 13 & 12 & 14 & 10 & 8 & 9 & 2 & 15\\
    \midrule
          & LR & 5 & 1 & 2 & 7 & 3 & 4 & 6 & 10 & 11 & 14 & 15 & 8 & 9 & 12 & 13\\
    Forex & XGB & 3 & 2 & 7 & 6 & 5 & 4 & 1 & 13 & 12 & 14 & 15 & 10 & 11 & 8 & 9\\
          & MLP & 1 & 6 & 5 & 11 & 3 & 4 & 2 & 13 & 12 & 14 & 15 & 7 & 10 & 8 & 9\\
    \midrule
          & LR & 5 & 12 & 9 & 3 & 2 & 1 & 8 & 7 & 11 & 10 & 13 & 4 & 6 & 14 & 15\\
    Heart & XGB & 2 & 10 & 11 & 5 & 4 & 3 & 1 & 8 & 12 & 9 & 14 & 6 & 7 & 13 & 15\\
          & MLP & 6 & 9 & 4 & 7 & 2 & 3  & 5 & 1 & 13 & 11 & 14 & 12 & 10 & 8 & 15\\
    \midrule
            & LR & 8 & 3 & 4 & 13 & 6 & 5 & 7 & 1 & 2 & 14 & 15 & 10 & 11 & 9 & 12\\
    Jasmine & XGB & 3 & 9 & 6 & 11 & 2 & 1 & 5 & 13 & 12 & 14 & 15 & 8 & 4 & 7 & 10\\
            & MLP & 11 & 12 & 1 & 2 & 8 & 9 & 7 & 13 & 10 & 14 & 15 & 4 & 5 & 3 & 6\\
    \midrule
             & LR & 8 & 4 & 7 & 13 & 1 & 2 & 3 & 10 & 12 & 14 & 15 & 5 & 6 & 9 & 11\\
    Madeline& XGB & 6 & 11 & 9 & 10 & 8 & 7 & 5 & 13 & 12 & 14 & 15 & 3 & 1 & 2 & 4\\
             & MLP & 6 & 9 & 8 & 5 & 11 & 10 & 7 & 12 & 13 & 14 & 15 & 2 & 3 & 1 & 4\\
    \midrule
                         & LR & 9 & 11 & 10 & 6 & 8 & 7 & 1 & 13 & 12 & 14 & 15 & 3 & 2 & 5 & 4\\
    \makecell{Pd\_speech\\ \_features} & XGB & 3 & 2 & 7 & 11 & 6 & 5 & 1 & 13 & 12 & 14 & 15 & 3 & 4 & 1 & 2\\
                         & MLP & 9 & 11 & 7 & 10 & 6 & 5 & 8 & 13 & 12 & 14 & 15 & 3 & 4 & 1 & 2\\
    \midrule
                  & LR & 4 & 6 & 8 & 1 & 11 & 3 & 10 & 2 & 15 & 5 & 9 & 12 & 13 & 7 & 14\\
    \makecell{Wine\\ \_quality} & XGB & 10 & 13 & 11 & 4 & 9 & 8 & 12 & 14 & 15 & 1 & 2 & 5 & 6 & 3 & 7\\
                  & MLP & 6 & 11 & 10 & 1 & 8 & 9 & 7 & 13 & 12 & 14 & 15 & 3 & 4 & 2 & 5\\
    \midrule
                      & LR & 6 & 9 & 5 & 14 & 3 & 2 & 1 & 12 & 15 & 8 & 10 & 4 & 7 & 11 & 13\\
    \makecell{Thyroid\\ \_allhyper} & XGB & 10 & 7 & 5 & 1 & 3 & 4 & 2 & 15 & 14 & 12 & 13 & 8 & 9 & 6 & 11\\
                      & MLP & 7 & 11 & 10 & 1 & 8 & 9 & 2 & 13 & 12 & 14 & 15 & 3 & 5 & 4 & 6\\
  \bottomrule
\end{tabular}
\end{table*}

\begin{table*}[t]% h asks to places the floating element [h]ere.
  \caption{Ranking on 10 datasets under 3600 seconds time constrain.}
  \label{tab:delta_acc_60_appendix}
  \footnotesize
  \begin{tabular}{p{0.06\textwidth}<{\centering}|
                  p{0.034\textwidth}<{\centering}|
                  p{0.03\textwidth}<{\centering}
                  p{0.034\textwidth}<{\centering}|
                  p{0.03\textwidth}<{\centering}
                  p{0.034\textwidth}<{\centering}|
                  p{0.04\textwidth}<{\centering}
                  p{0.04\textwidth}<{\centering}
                  p{0.032\textwidth}<{\centering}|
                  p{0.054\textwidth}<{\centering}
                  p{0.034\textwidth}<{\centering}|
                  p{0.06\textwidth}<{\centering}
                  p{0.035\textwidth}<{\centering}|
                  p{0.03\textwidth}<{\centering}
                  p{0.03\textwidth}<{\centering}
                  p{0.03\textwidth}<{\centering}
                  p{0.035\textwidth}<{\centering}}
    \toprule
    Dataset & ML Model & RS & Anneal & TPE & SMAC & TEVO\_H & TEVO\_Y & PBT & REINFORCE & ENAS & HYPERBAND & BOHB & PMNE & PME & PLNE & PLE \\
    \midrule
               & LR & 4 & 14 & 9 & 13 & 6 & 5 & 3 & 8 & 11 & 7 & 10 & 1 & 2 & 12 & 15\\
    Austrilian & XGB & 1 & 15 & 8 & 11 & 9 & 7 & 2& 12 & 14 & 5 & 10 & 3 & 4 & 6 & 13\\
               & MLP & 4 & 11 & 13 & 7 & 1 & 5 & 6 & 10 & 15 & 9 & 12 & 2 & 3 & 8 & 14\\
    \midrule
          & LR & 7 & 12 & 10 & 13 & 5 & 2 & 1 & 14 & 15 & 6 & 9 & 3 & 4 & 8 & 11 \\
    Blood & XGB & 3 & 15 & 10 & 8 & 6 & 7 & 4 & 12 & 13 & 5 & 14 & 1 & 2 & 9 & 11\\
          & MLP & 11 & 14 & 4 & 9 & 2 & 5 & 1 & 12 & 15 & 6 & 13 & 3 & 7 & 8 & 10\\
    \midrule
            & LR & 3 & 13 & 10 & 11 & 4 & 2 & 1 & 9 & 15 & 7 & 12 & 5 & 6 & 8 & 14\\
    Emotion & XGB & 4 & 13 & 6 & 9 & 3 & 1 & 2 & 7 & 15 & 10 & 12 & 8 & 5 & 11 & 14\\
            & MLP & 3 & 14 & 6 & 7 & 2 & 1 & 5 & 4 & 15 & 11 & 10 & 9 & 12 & 8 & 13\\
    \midrule
          & LR & 7 & 12 & 6 & 2 & 11 & 10 & 1 & 8 & 15 & 9 & 13 & 3 & 4 & 5 & 14\\
    Forex & XGB & 11 & 14 & 6 & 4 & 2 & 1 & 3 & 5 & 15 & 7 & 8 & 10 & 9 & 13 & 12\\
          & MLP & 5 & 10 & 9 & 6 & 2 & 7 & 1 & 11 & 14 & 3 & 4 & 12 & 13 & 8 & 15\\
    \midrule
          & LR & 3 & 13 & 6 & 10 & 8 & 5 & 4 & 11 & 14 & 7 & 12 & 1 & 2 & 9 & 15\\
    Heart & XGB & 6 & 15 & 10 & 11 & 7 & 9 & 4 & 1 & 14 & 5 & 12 & 3 & 2 & 8 & 13\\
          & MLP & 2 & 15 & 6 & 9 & 5 & 4 & 1 & 3 & 14 & 12 & 13 & 8 & 7 & 11 & 10\\
    \midrule
            & LR & 2 & 15 & 5 & 12 & 1 & 6 & 3 & 4 & 14 & 10 & 11 & 8 & 7 & 9 & 13\\
    Jasmine & XGB & 4 & 7 & 8 & 11 & 1 & 5 & 2 & 3 & 15 & 13 & 14 & 10 & 9 & 6 & 12\\
            & MLP & 2 & 12 & 10 & 11 & 1 & 5 & 4 & 6 & 15 & 13 & 14 & 8 & 9 & 3 & 7\\
    \midrule
             & LR & 9 & 12 & 10 & 5 & 1 & 2 & 3 & 6 & 11 & 13 & 14 & 8 & 7 & 4 & 15\\
    Madeline& XGB & 1 & 9 & 12 & 7 & 10 & 6 & 4 & 8 & 15 & 5 & 14 & 2 & 3 & 13 & 11\\
             & MLP & 4 & 8 & 7 & 5 & 6 & 3 & 1 & 2 & 15 & 13 & 9 & 11 & 12 & 10 & 14\\
    \midrule
                         & LR & 7 & 11 & 8 & 9 & 6 & 4 & 5 & 15 & 14 & 13 & 12 & 1 & 2 & 3 & 10\\
    \makecell{Pd\_speech\\ \_features} & XGB & 8 & 13 & 9 & 11 & 6 & 3 & 2 & 12 & 15 & 11 & 14 & 5 & 7 & 4 & 10\\
                         & MLP & 6 & 13 & 7 & 8 & 9 & 10 & 3 & 14 & 15 & 12 & 11 & 1 & 2 & 4 & 5\\
    \midrule
                  & LR & 4 & 15 & 5 & 6 & 14 & 12 & 1 & 9 & 10 & 11 & 13 & 2 & 3 & 7 & 8\\
    \makecell{Wine\\ \_quality} & XGB & 6 & 14 & 10 & 3 & 12 & 11 & 13 & 1 & 15 & 7 & 9 & 5 & 8 & 2 & 4\\
                  & MLP & 1 & 13 & 12 & 10 & 7 & 6 & 8 & 14 & 15 & 9 & 11 & 3 & 5 & 4 & 2\\
    \midrule
                      & LR & 5 & 15 & 10 & 11 & 6 & 3 & 7 & 4 & 12 & 9 & 14 & 2 & 1 & 8 & 13\\
    \makecell{Thyroid\\ \_allhyper} & XGB & 11 & 14 & 10 & 12 & 1 & 3 & 2 & 6 & 15 & 13 & 8 & 5 & 4 & 9 & 7\\
                      & MLP & 8 & 14 & 9 & 4 & 1 & 3 & 2 & 11 & 15 & 12 & 13 & 6 & 5 & 7 & 10\\
  \bottomrule
\end{tabular}
\end{table*}

\begin{table*}[t]% h asks to places the floating element [h]ere.
  \caption{$|\Delta \ Acc|$ between best algorithm with 3600 seconds time constrain and other time constrains.}
  \label{tab:delta_acc_3600_with_others}
  \begin{tabular}{p{0.3\linewidth}<{\centering}
                  p{0.12\linewidth}<{\centering}
                  p{0.12\linewidth}<{\centering}
                  p{0.12\linewidth}<{\centering}
                  p{0.12\linewidth}<{\centering}}
    \toprule
    \textbf{Dataset} & \textbf{Time} & \textbf{LR} & \textbf{XGB} & \textbf{MLP}\\ 
    \midrule
               & 60 & 0.9 & 0.90 & 0.90\\ 
               & 300 & 0.72 & 0.18 & 0.54\\ 
    Austrilian & 600 & 0.18 & 0.18 & 0.54\\ 
               & 1200 & 0.00 & 0.18 & 0.36\\ 
               & 1800 & 0.00 & 0.18 & 0.36\\ 
    \midrule
          & 60 & 0.00 & 1.17 & 0.50\\ 
          & 300 & 0.00 & 1.00 & 0.33\\ 
    Blood & 600 & 0.00 & 0.50 & 0.33\\ 
          & 1200 & 0.00 & 0.50 & 0.33\\ 
          & 1800 & 0.00 & 0.17 & 0.17\\ 
    \midrule
            & 60 & 3.49 & 2.86 & 3.81\\ 
            & 300 & 1.27 & 0.32 & 2.86\\ 
    Emotion & 600 & 0.63 & 0.00 & 1.90\\ 
            & 1200 & 0.00 & 0.00 & 1.90\\ 
            & 1800 & 0.00 & 0.00 & 1.59\\ 
    \midrule
          & 60 & 4.07 & 3.77 & 9.43\\ 
         & 300 & 0.39 & 3.31 & 4.09\\ 
    Forex & 600 & 0.00 & 1.73 & 4.80\\ 
          & 1200 & 0.00 & 0.93 & 2.60\\ 
          & 1800 & 0.00 & 0.01 & 2.38\\ 
    \midrule
          & 60 & 1.63 & 2.45 & 4.49\\ 
          & 300 & 1.22 & 1.63 & 2.45\\ 
    Heart & 600 & 0.41 & 0.82 & 1.63\\ 
          & 1200 & 0.41 & 0.00 & 0.41\\ 
          & 1800 & 0.41 & 0.00 & 0.41\\ 
    \midrule
            & 60 & 0.88 & 1.46 & 1.21\\ 
            & 300 & 0.50 & 0.75 & 0.67\\ 
    Jasmine & 600 & 0.46 & 0.46 & 0.50\\ 
            & 1200 & 0.25 & 0.25 & 0.08\\ 
            & 1800 & 0.17 & 0.25 & 0.00\\ 
    \midrule
             & 60 & 3.78 & 0.99 & 5.41\\ 
             & 300 & 1.43 & 0.32 & 2.43\\ 
    Madeline & 600 & 1.43 & 0.20 & 2.43\\ 
             & 1200 & 1.43 & 0.16 & 1.23\\ 
             & 1800 & 1.43 & 0.08 & 0.48\\ 
    \midrule
                       & 60 & 1.49 & 3.31 & 2.31\\ 
                       & 300 & 0.17 & 1.65 & 0.66\\ 
    Pd\_speech\_features & 600 & 0.00 & 0.99 & 0.33\\ 
                       & 1200 & 0.00 & 0.17 & 0.33\\ 
                       & 1800 & 0.00 & 0.17 & 0.00\\ 
    \midrule
                 & 60 & 0.94 & 1.08 & 0.83\\ 
                 & 300 & 0.13 & 1.02 & 0.42\\ 
    Wine\_quality & 600 & 0.04 & 0.77 & 0.23\\ 
                 & 1200 & 0.00 & 0.62 & 0.13\\ 
                 & 1800 & 0.00 & 0.56 & 0.13\\ 
    \midrule
                     & 60 & 0.40 & 1.65 & 1.07\\ 
                     & 300 & 0.04 & 0.62 & 0.76\\ 
    Thyroid-allhyper & 600 & 0.04 & 0.62 & 0.36\\ 
                     & 1200 & 0.00 & 0.45 & 0.18\\ 
                     & 1800 & 0.00 & 0.13 & 0.18\\
    \bottomrule
  \end{tabular}
\end{table*}

\end{appendix}
